# Supplementary material for: Exploring the short-term variability of H$\alpha$ and H$\beta$ emissions in a sample of M dwarfs
Source: arXiv:2307.11574 source file (2023-07-21)
Supplement: Supplementary file 1 [file Supplementary_material_MDwarf_H-alpha_Variability_MNRAS.pdf]

# 1 Supplementary Material

## 1.1 Appendix-I

The figure shows the spectral times series (panel a), photometric light curves from TESS and Kepler/K2 databases (panel b), EWs light curves for H$\alpha$ and H$\beta$ emissions (panel c) and their computed fractional structure functions (SFs) (panel d) for each of the sources observed with MFOSC-P instrument on PRL 1.2m telescope at Mt. Abu. Source ID, spectral type, and rotation period are also mentioned at the top of the panel (a). Data for H$\alpha$ and H$\beta$ are shown in red circles and black triangles, respectively. The Y-axis (ordinate) of panel (a) is in arbitrary units of flux. Y-axes of panel (c) are in units of Å for H$\alpha$ (left) and H$\beta$ (right). Y-axes of the panel (d) are the fractional structure function (SF) for H$\alpha$ (left) and H$\beta$ (right). Units of X-axes (abscissa) of the panel (a), (c), and (d) are given at the bottom of these plots. The X-axis of the panel (b) - photometric light curves - is in units of days, and Y-axis is in arbitrary units of flux. See Fig.4 of the main text also for these units. For some sources, either light curves were not found or rotation periods could not be determined, and/or H$\beta$ emission was not covered. Thus, these data are not presented for some of the sources.

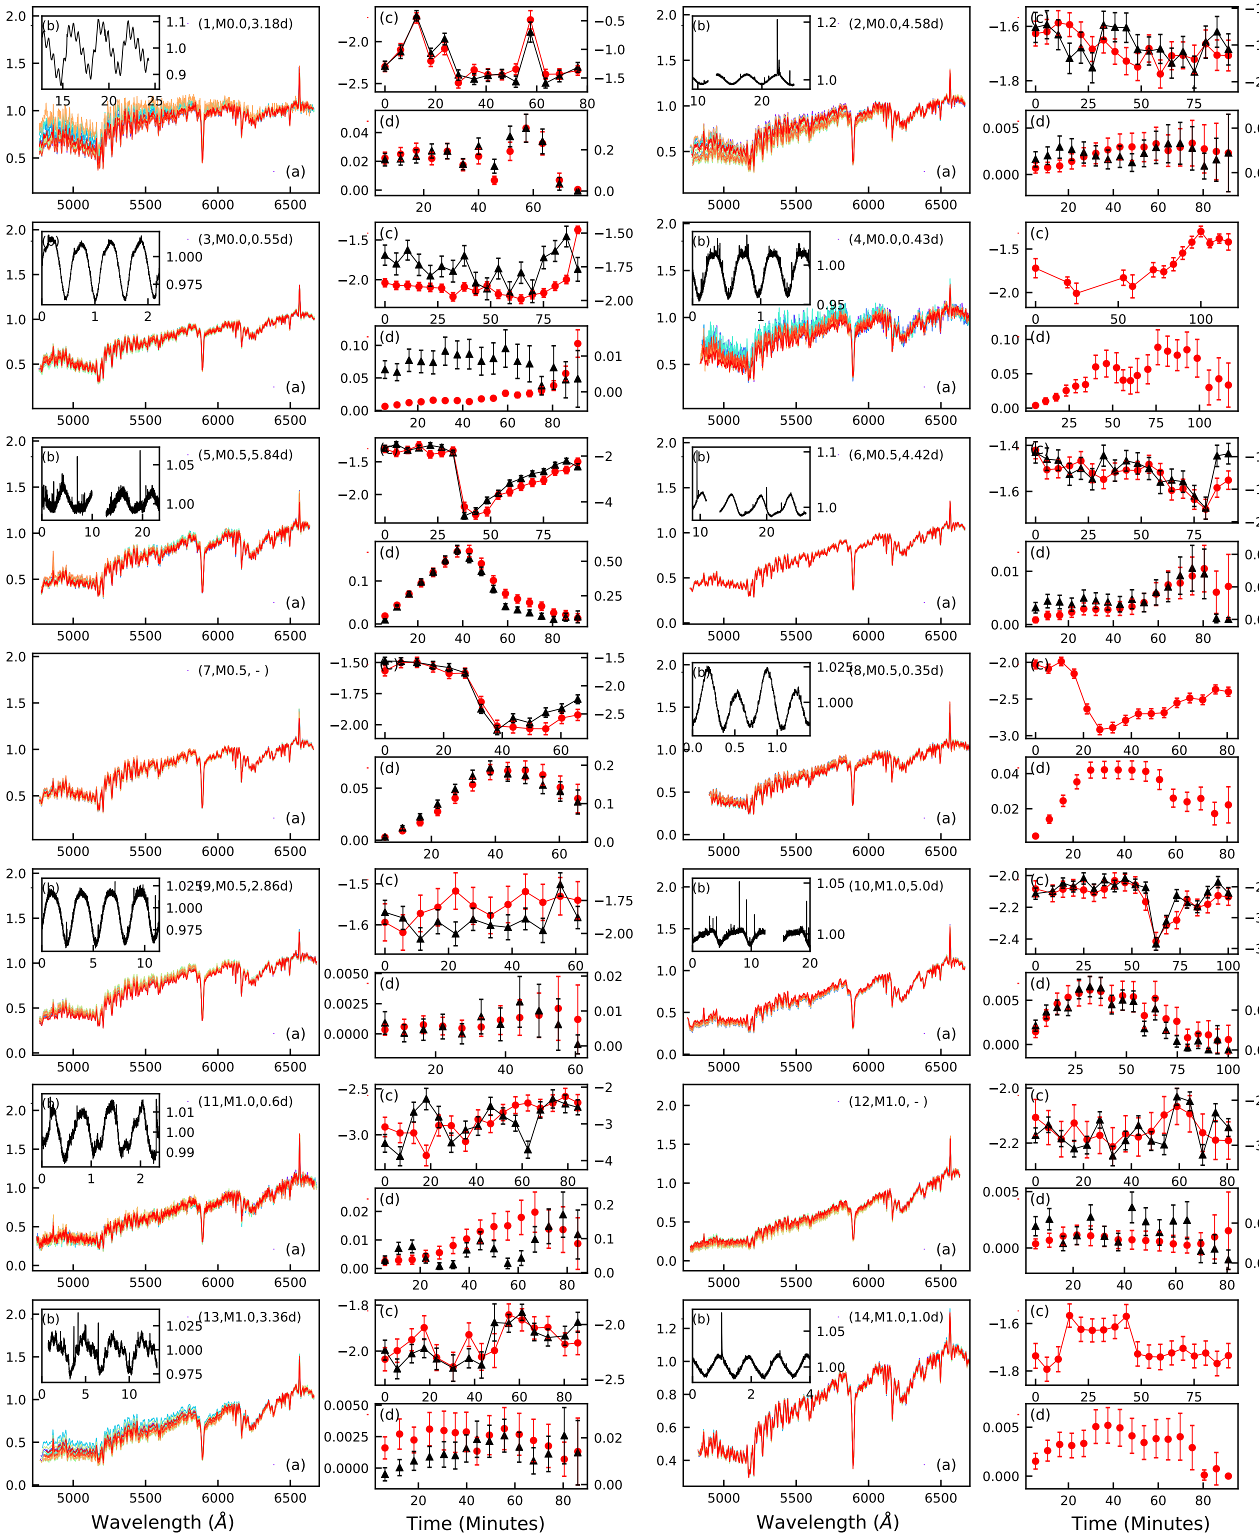


Figure 1: The figure shows the spectral times series (panel a), photometric light curves from TESS and Kepler/K2 databases (panel b), EWs light curves for H$\alpha$ and H$\beta$ emissions (panel c) and their computed fractional structure functions (SFs) (panel d) for each of the sources (full caption is given in the Appendix-I text).

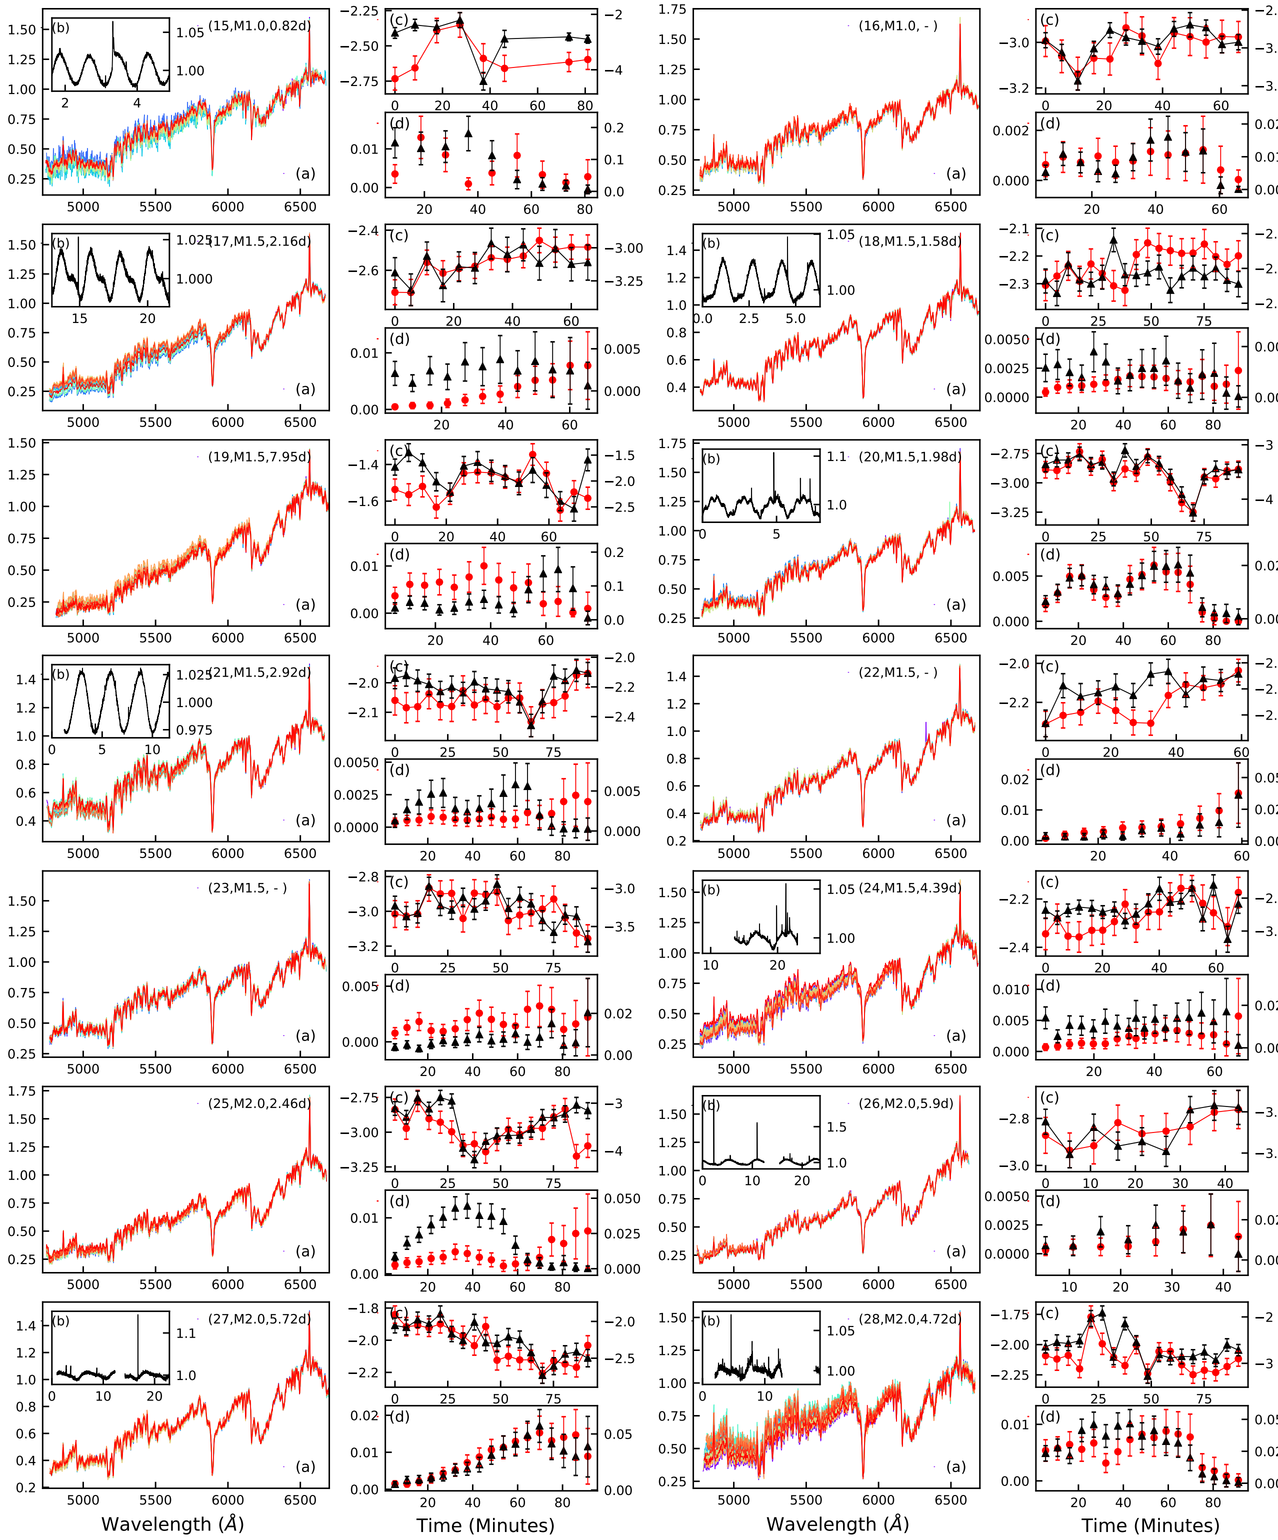


Figure 1: Continue...

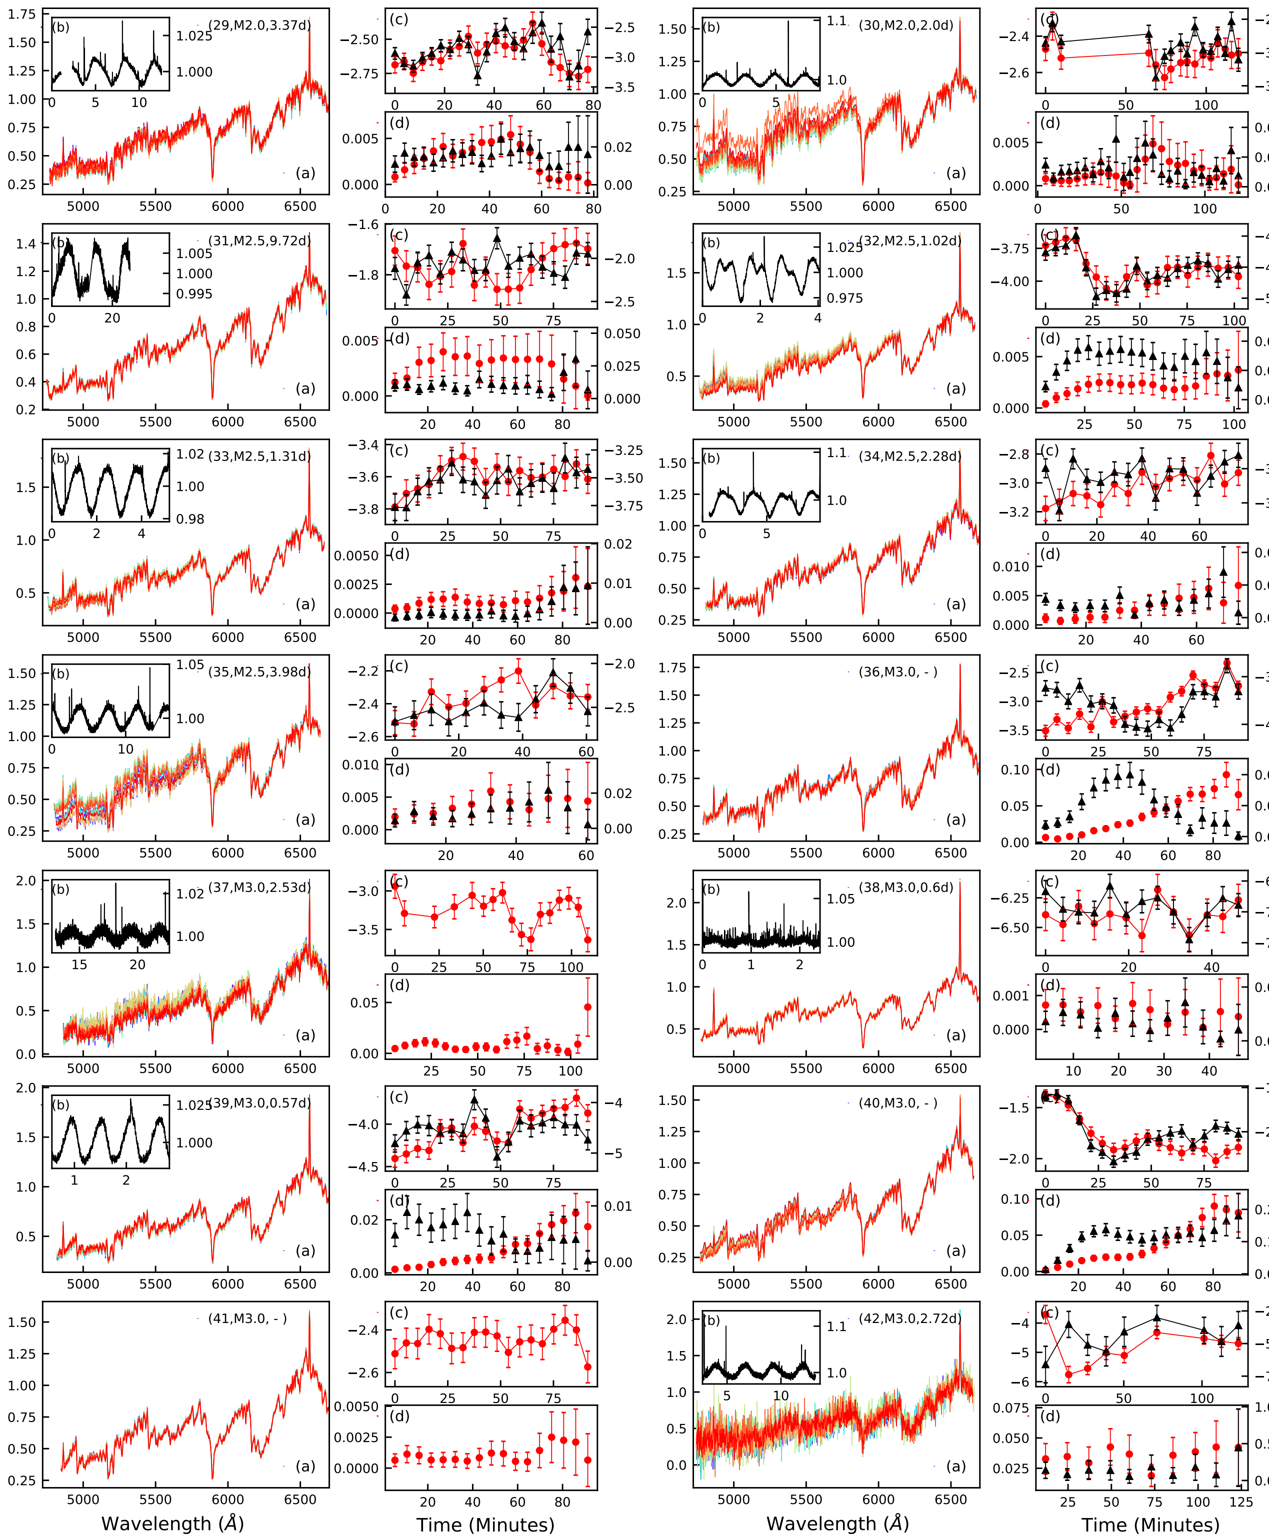


Figure 1: Continue...

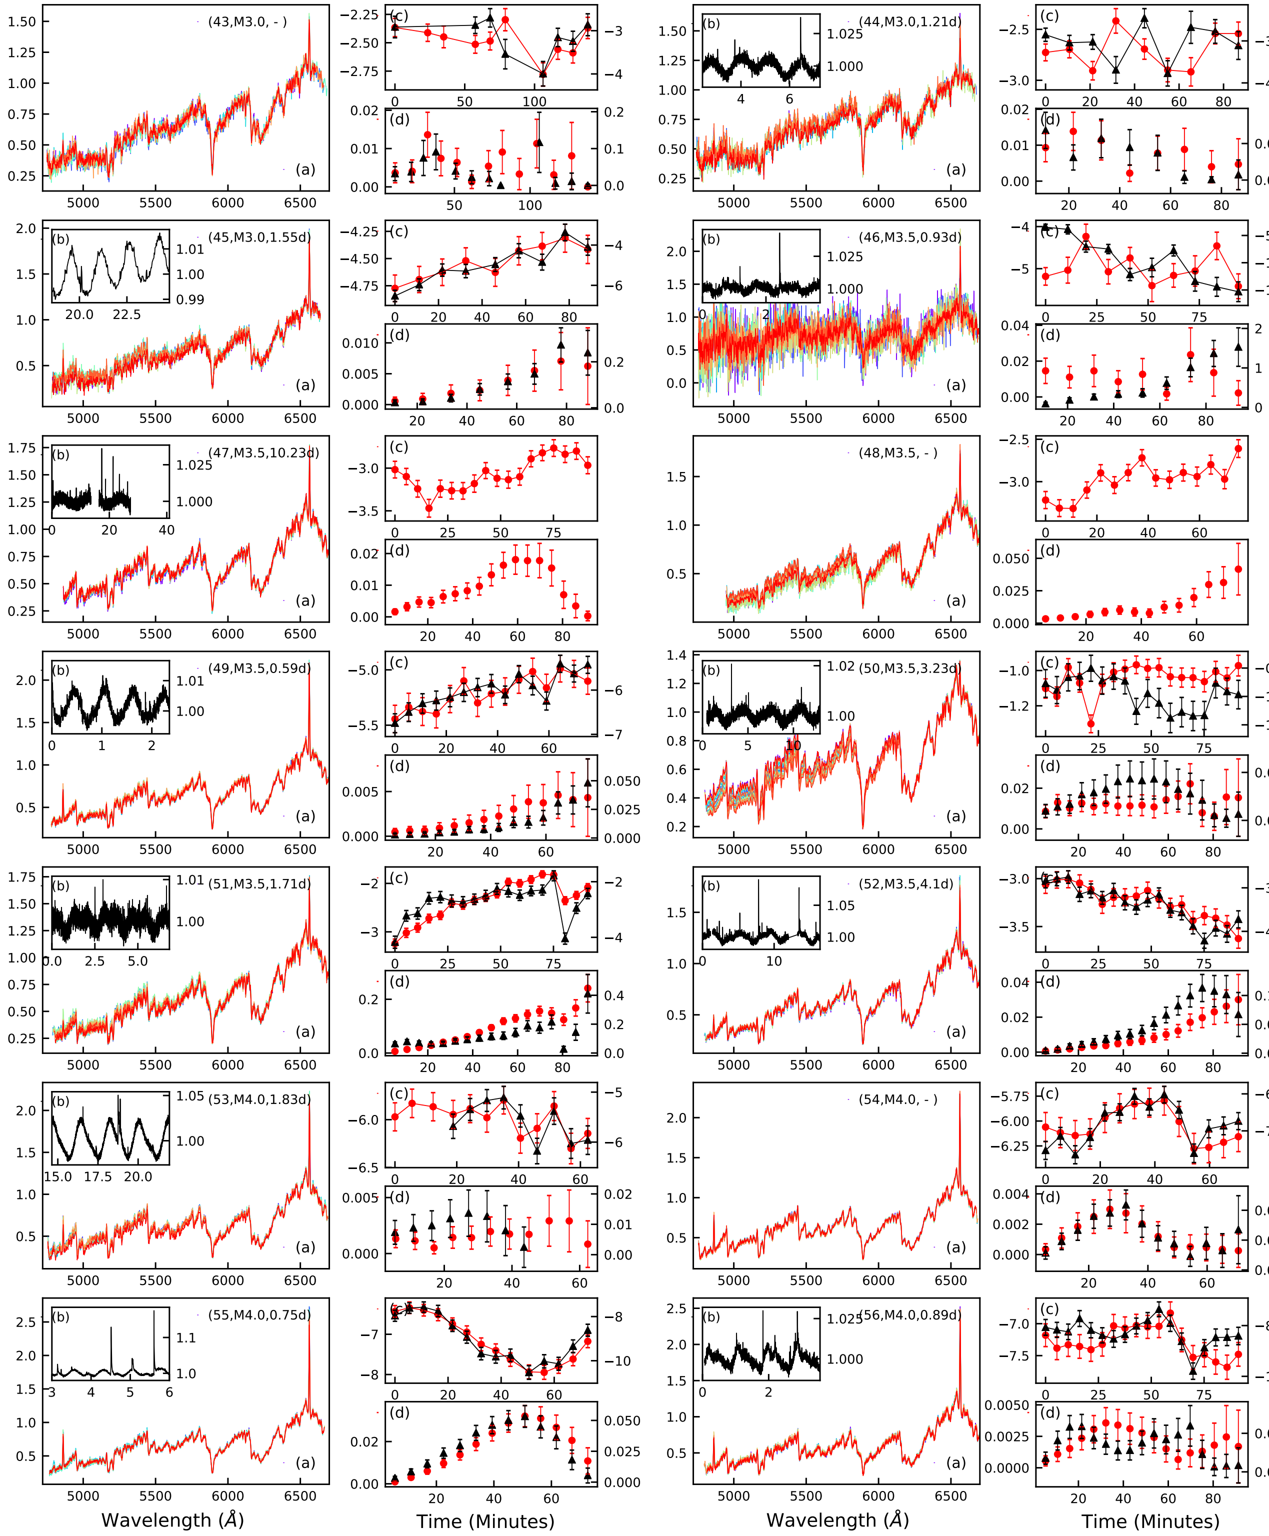


Figure 1: Continue...

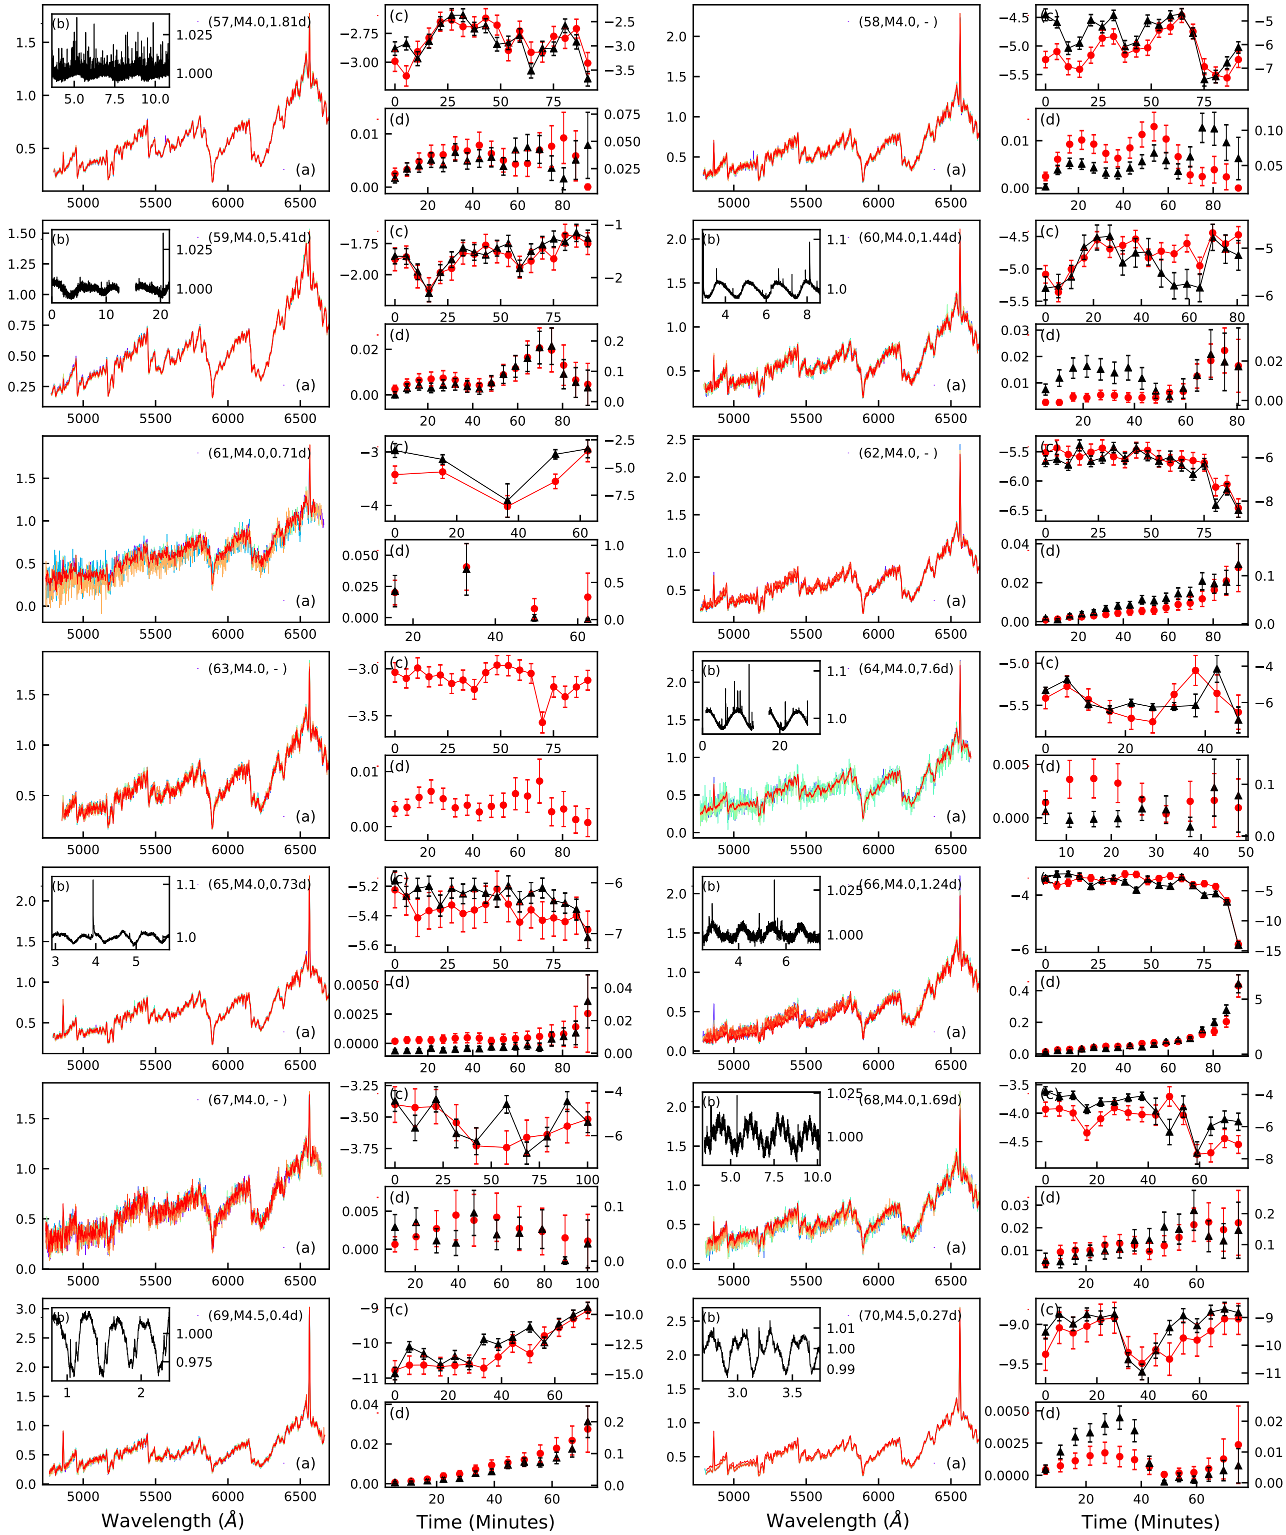


Figure 1: Continue...

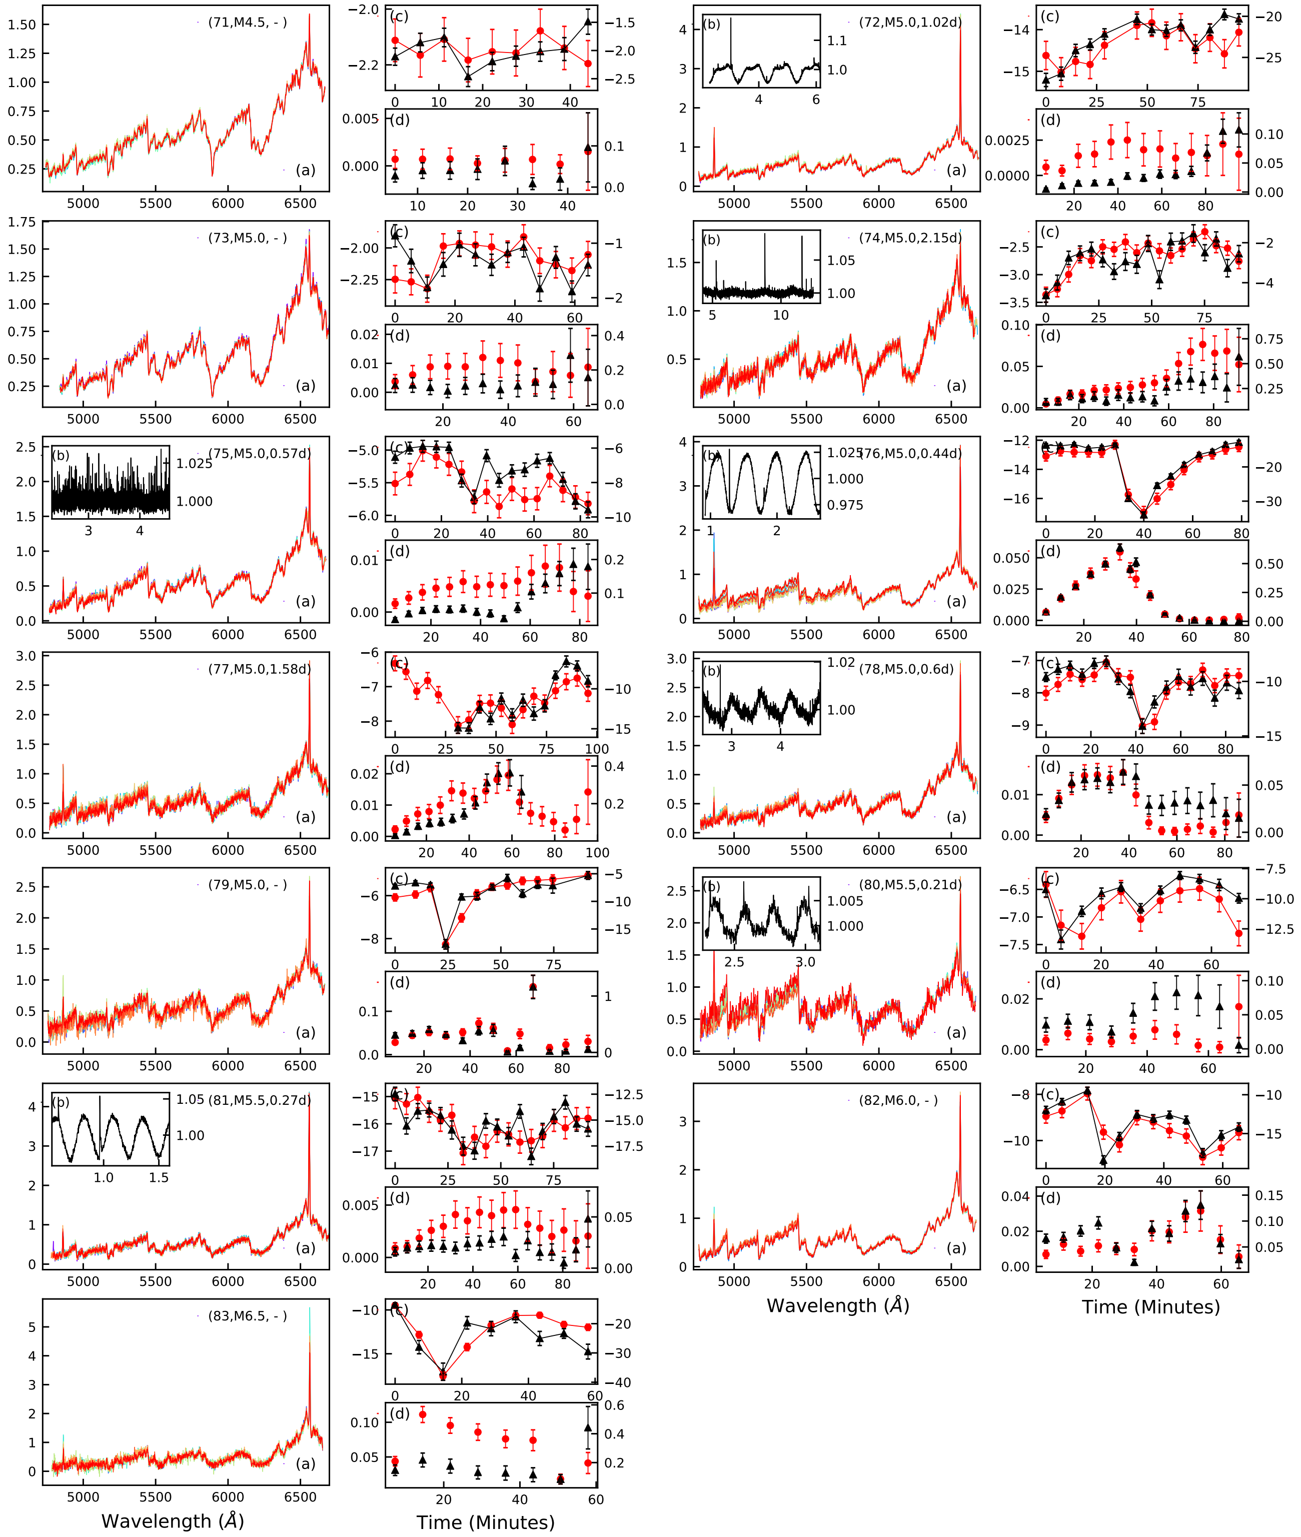


Figure 1: Continue...

## 1.2 Appendix-II

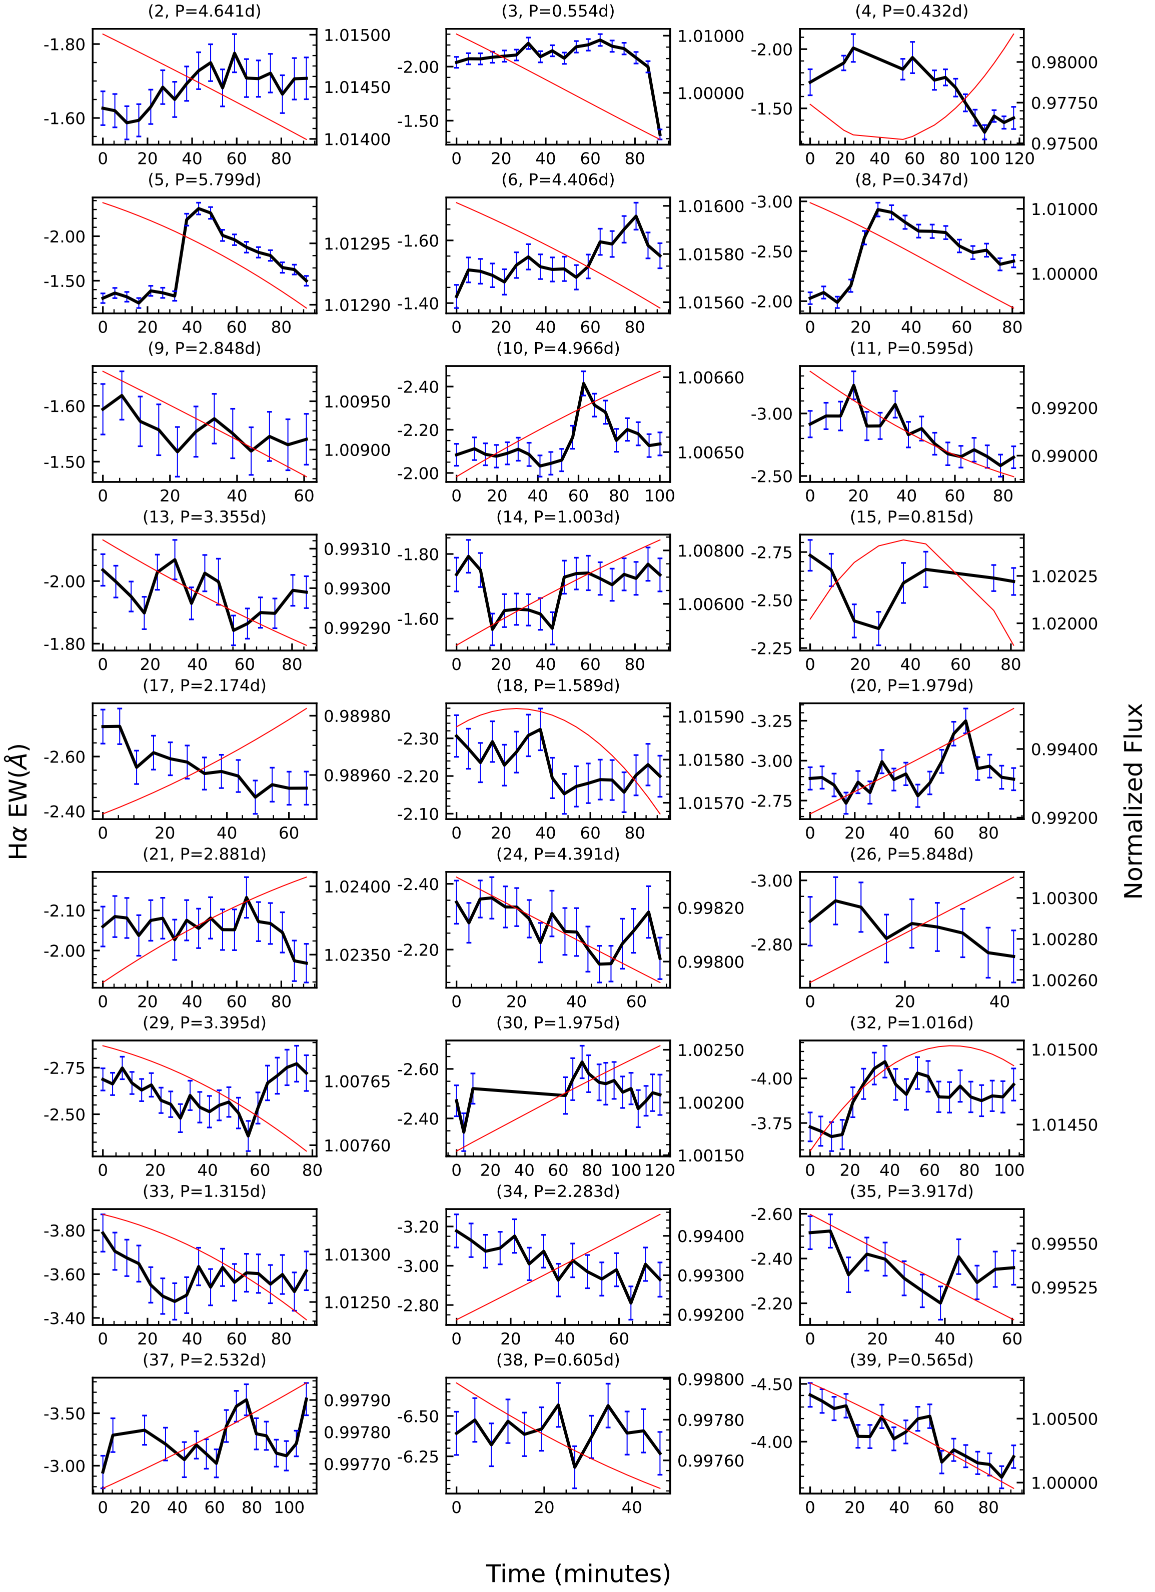


Figure 2: The figure shows the Hα Equivalent Width (EW) light curve (black data points) and corresponding extrapolated photometric light curve (red line; from TESS and Kepler/K2 databases). Source ID and rotation period are also mentioned at the top of each panel. The left Y-axis of each panel is the Hα EW in the units of Å and the right Y-axis is the full phase mean normalized flux. The X-axis of each panel is the time in units of minutes, taking reference as the starting of our spectroscopic monitoring observation.

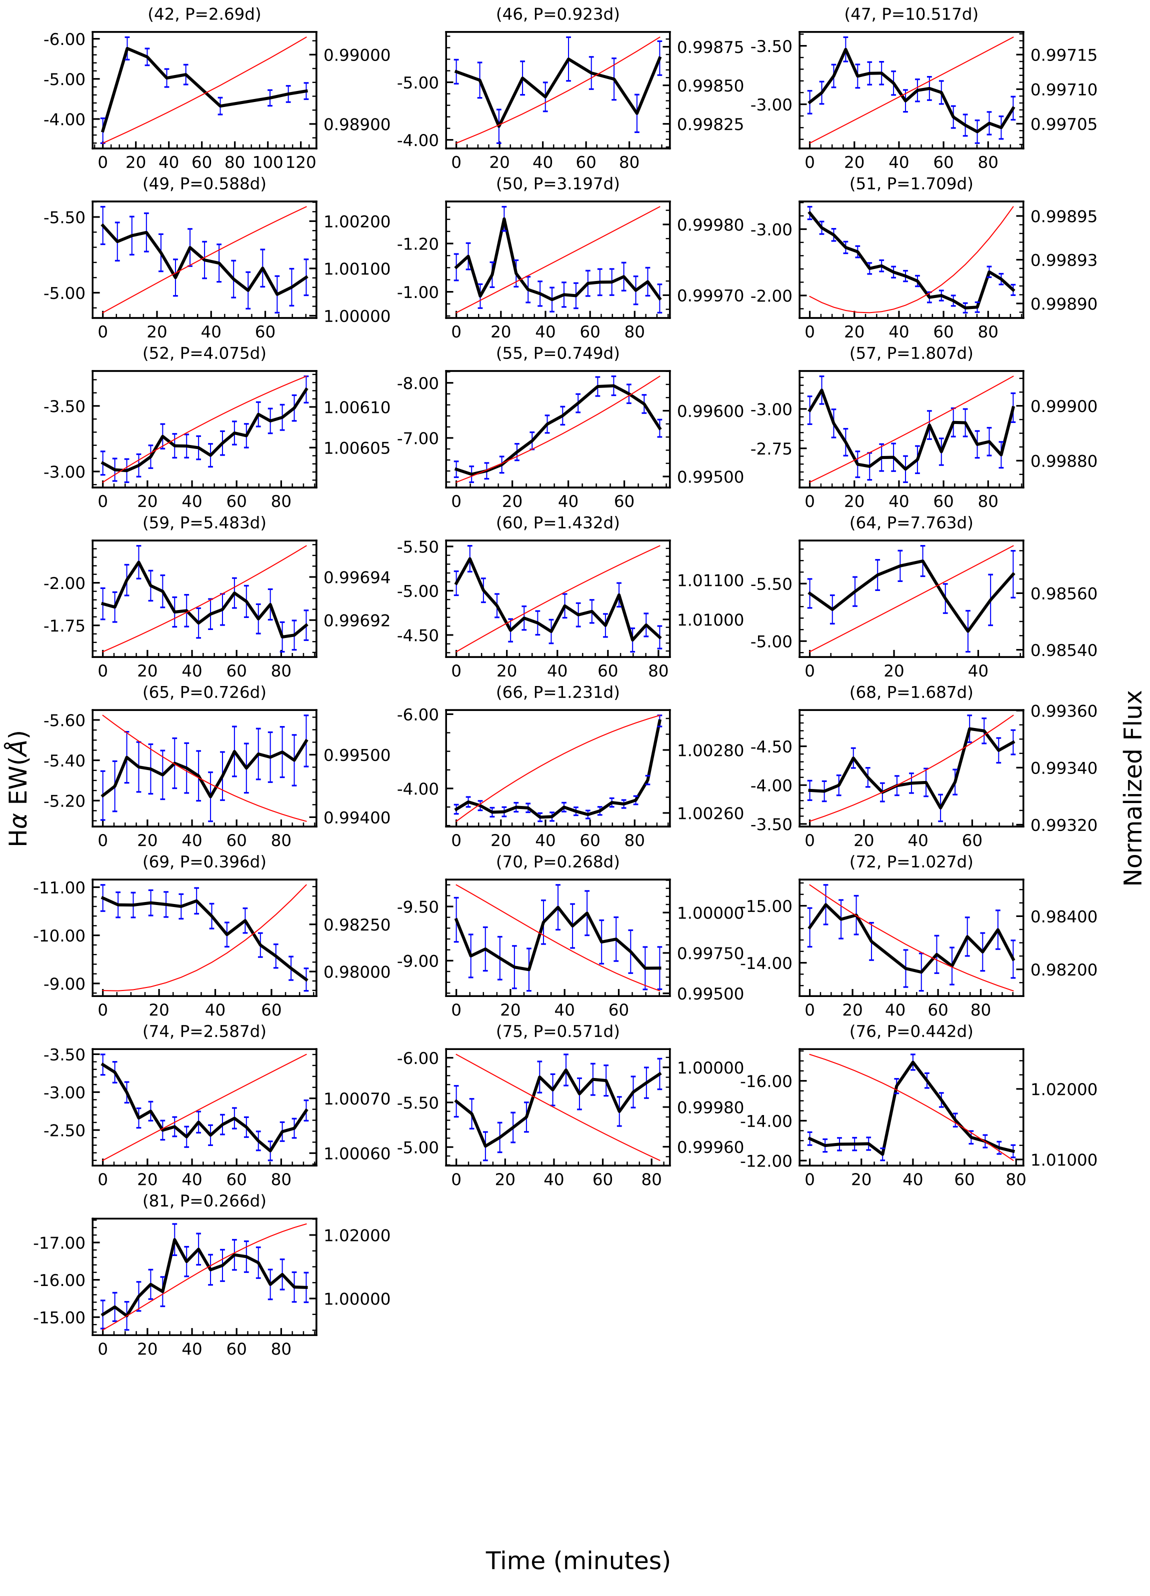


Figure 2: Continue...

## 1.3 Appendix-III

Table 1: Observation details of the sources of this study along with the derived stellar parameters. V band magnitudes are taken from the SIMBAD database. The spectral types are mostly taken from Lépine et al. (2013), and Jeffers et al. (2018), except for six sources where we have derived the spectral class. These sources are marked with (⋆).

| Source ID | Source name | Spectral type | Magnitude (V-band) | Date of observation (UT) | Frame exposure time × No. of frames (s) | log g (cm $s^{-2}$) | $T_{eff}$ (K) |
|---|---|---|---|---|---|---|---|
| 1 | PM J03332+4615S | M0.0 | 13.09 | 2020-12-29.602 | 300sx14 | 5.0 | 3900 |
| 2 | PM J03416+5513 | M0.0 | - | 2021-02-01.600 | 300sx18 | 5.0 | 3800 |
| 3 | PM J07151+1555 | M0.0 | 11.37 | 2021-01-30.754 | 300sx18 | 5.0 | 4000 |
| 4 | PM J23083-1524 | M0.0 | 10.87 | 2020-11-26.563 | 300sx14 | 4.5 | 3900 |
| 5 | PM J03322+4914S | M0.5 | 11.94 | 2021-02-03.680 | 300sx18 | 5.0 | 3700 |
| 6 | PM J04595+0147 | M0.5 | 10.11 | 2021-01-31.618 | 300sx18 | 5.0 | 3900 |
| 7 | PM J10143+2104 | M0.5 | 10.08 | 2020-12-29.882 | 300sx13 | 5.0 | 3800 |
| 8 | PM J19026+3231 | M0.5 | 11.57 | 2021-03-23.963 | 300sx16 | 5.0 | 3700 |
| 9 | PM J23060+6355 | M0.5 | 10.96 | 2020-12-27.599 | 300sx12 | 5.0 | 3700 |
| 10 | PM J06310+5002 | M1.0 | - | 2021-01-31.711 | 300sx19 | 5.0 | 3700 |
| 11 | PM J08317+0545 | M1.0 | 11.93 | 2021-01-30.854 | 300sx16 | 5.0 | 3800 |
| 12 | PM J09193+6203 | M1.0 | - | 2021-03-08.811 | 300sx16 | 5.5 | 3600 |
| 13 | PM J12576+3513E | M1.0 | - | 2020-03-20.846 | 300sx15 | 5.0 | 3600 |
| 14 | PM J15238+5609 | M1.0 | 11.68 | 2021-03-22.832 | 300sx18 | 5.0 | 3800 |
| 15 | PM J15581+4927 | M1.0 | - | 2020-05-06.890 | 450sx8 | 5.5 | 3600 |
| 16 | PM J04376-0229 | M1.0 | 10.59 | 2020-12-29.755 | 300sx13 | 5.0 | 3600 |
| 17 | PM J00428+3532 | M1.5 | - | 2020-12-29.679 | 300sx13 | 5.0 | 3500 |
| 18 | PM J05402+1239 | M1.5 | 11.35 | 2021-03-02.606 | 300sx18 | 5.0 | 3700 |
| 19 | PM J06262+2349 | M1.5 | 11.82 | 2021-03-26.681 | 300sx15 | 5.0 | 3500 |
| 20 | PM J07295+3556 | M1.5 | 11.88 | 2021-02-03.787 | 300sx18 | 5.0 | 3600 |
| 21 | PM J13007+1222 | M1.5 | 9.75 | 2021-01-31.905 | 300sx18 | 4.5 | 3900 |
| 22 | PM J15416+1828 | M1.5 | 12.32 | 2021-02-01.007 | 300sx12 | 5.0 | 3600 |
| 23 | PM J16220+2250 | M1.5 | 12.12 | 2021-03-25.850 | 300sx18 | 5.0 | 3700 |
| 24 | PM J22387-2037 | M1.5 | 9.08 | 2020-12-02.626 | 200sx18 | 5.0 | 3600 |
| 25 | PM J04284+1741 | M2.0 | 12.12 | 2021-02-01.683 | 300sx18 | 5.0 | 3500 |
| 26 | PM J06212+4414 | M2.0 | - | 2021-01-31.825 | 300sx9 | 5.0 | 3500 |
| 27 | PM J11201-1029 | M2.0 | 11.25 | 2021-03-23.772 | 300sx18 | 5.0 | 3500 |
| 28 | PM J13518+1247 | M2.0 | 12.25 | 2021-02-01.940 | 300sx18 | 5.0 | 3800 |
| 29 | PM J15218+2058 | M2.0 | 10.00 | 2021-03-08.973 | 200sx22 | 5.0 | 3600 |
| 30 | PM J16170+5516 | M2.0 | 9.46 | 2020-05-06.752 | 200sx16 | 5.0 | 3600 |
| 31 | PM J06596+0545 | M2.5 | 12.50 | 2021-02-01.764 | 300sx18 | 5.0 | 3500 |
| 32 | PM J09177+4612 | M2.5 | 11.58 | 2021-01-28.857 | 300sx20 | 5.0 | 3500 |
| 33 | PM J10043+5023 | M2.5 | - | 2021-02-01.851 | 300sx18 | 5.0 | 3500 |
| 34 | PM J11519+0731 | M2.5 | 12.42 | 2021-03-08.902 | 300sx15 | 5.0 | 3500 |
| 35 | PM J15557+6840 | M2.5 | 11.97 | 2020-05-22.902 | 300sx12 | 5.0 | 3400 |
| 36 | PM J04333+2359 | M3.0 | 12.66 | 2021-02-02.597 | 300sx18 | 4.5 | 3500 |
| 37 | PM J05091+1527 | M3.0 | - | 2021-02-02.685 | 300sx17 | 5.0 | 3400 |
| 38 | PM J05337+0156 | M3.0 | 11.50 | 2020-11-27.854 | 200sx13 | 5.0 | 3400 |
| 39 | PM J05547+1055 | M3.0 | - | 2021-03-27.613 | 300sx18 | 4.5 | 3500 |
| 40 | PM J07319+3613S | M3.0 | - | 2021-03-25.611 | 300sx18 | 5.0 | 3400 |
| 41 | PM J07349+1445 | M3.0 | 11.15 | 2021-02-02.786 | 300sx18 | 5.0 | 3400 |
| 42 | PM J11529+3554⋆ | M3.0 | 13.69 | 2020-05-21.751 | 600sx9 | 5.0 | 3300 |
| 43 | PM J12355+2439⋆ | M3.0 | 13.43 | 2020-03-08.784 | 600sx10 | 5.0 | 3500 |
| 44 | PM J13352+1714⋆ | M3.0 | 13.19 | 2020-05-24.730 | 600sx9 | 5.0 | 3600 |
| 45 | PM J14137+4618⋆ | M3.0 | 13.14 | 2020-05-21.873 | 600sx9 | 5.0 | 3400 |
| 46 | PM J04238+1455 | M3.5 | 13.35 | 2020-11-26.785 | 500sx10 | 4.5 | 3500 |
| 47 | PM J09302+2630 | M3.5 | - | 2021-02-02.870 | 300sx18 | 4.5 | 3400 |
| 48 | PM J09557+3521 | M3.5 | - | 2021-02-02.967 | 300sx15 | 5.0 | 3300 |
| 49 | PM J12485+4933 | M3.5 | 12.51 | 2021-02-03.977 | 300sx15 | 5.0 | 3400 |

Table 1: continue...

| Source ID | Source name | Spectral type | Magnitude (V-band) | Date of observation (UT) | Frame exposure time × No. of frames (s) | log g (cm $s^{-2}$) | $T_{eff}$ (K) |
|---|---|---|---|---|---|---|---|
| 50 | PM J12490+6606 | M3.5 | - | 2021-03-26.764 | 300sx18 | 4.5 | 3500 |
| 51 | PM J13417+5815 | M3.5 | 12.54 | 2021-03-23.871 | 300sx18 | 5.0 | 3300 |
| 52 | PM J16591+2058 | M3.5 | 12.45 | 2021-03-26.892 | 300sx18 | 5.0 | 3400 |
| 53 | PM J00325+0729 | M4.0 | 12.80 | 2020-11-27.723 | 300sx12 | 4.5 | 3200 |
| 54 | PM J01593+5831 | M4.0 | 12.15 | 2020-11-27.786 | 300sx14 | 5.0 | 3200 |
| 55 | PM J02088+4926 | M4.0 | 12.45 | 2020-12-02.827 | 300sx14 | 5.0 | 3300 |
| 56 | PM J05062+0439 | M4.0 | 13.46 | 2021-02-12.597 | 300sx18 | 4.0 | 3200 |
| 57 | PM J06000+0242 | M4.0 | 11.31 | 2021-03-26.601 | 300sx18 | 5.0 | 3200 |
| 58 | PM J07033+3441 | M4.0 | - | 2021-02-12.685 | 300sx18 | 5.0 | 3200 |
| 59 | PM J07100+3831 | M4.0 | 11.52 | 2021-03-27.697 | 300sx18 | 5.0 | 3100 |
| 60 | PM J09161+0153 | M4.0 | 13.03 | 2021-02-24.75 | 300sx16 | 5.0 | 3300 |
| 61 | PM J10357+0215⋆ | M4.0 | 13.57 | 2020-05-22.665 | 600sx5 | 5.0 | 3400 |
| 62 | PM J10360+0507 | M4.0 | 12.64 | 2021-02-23.784 | 300sx18 | 5.0 | 3300 |
| 63 | PM J11033+1337 | M4.0 | - | 2021-03-24.744 | 300sx18 | 5.0 | 3300 |
| 64 | PM J11118+3332S | M4.0 | - | 2021-02-24.827 | 300sx10 | 5.0 | 3300 |
| 65 | PM J12156+5239 | M4.0 | 12.56 | 2021-02-12.863 | 300sx18 | 5.0 | 3400 |
| 66 | PM J13536+7737 | M4.0 | - | 2021-02-12.971 | 300sx18 | 5.0 | 3100 |
| 67 | PM J14165-0725⋆ | M4.0 | 13.76 | 2020-05-22.806 | 600sx10 | 4.5 | 3400 |
| 68 | PM J15126+4543 | M4.0 | 13.33 | 2021-02-24.975 | 300sx15 | 5.0 | 3200 |
| 69 | PM J05243-1601 | M4.5 | 13.57 | 2020-12-02.899 | 300sx14 | 4.0 | 3000 |
| 70 | PM J13317+2916 | M4.5 | 12.02 | 2021-02-24.900 | 300sx15 | 5.0 | 3200 |
| 71 | PM J17199+2630W | M4.5 | 11.34 | 2020-05-21.956 | 300sx9 | 5.0 | 3200 |
| 72 | PM J01033+6221 | M5.0 | 13.21 | 2020-11-28.675 | 400sx13 | 4.0 | 3000 |
| 73 | PM J02002+1303 | M5.0 | 12.30 | 2021-02-23.597 | 300sx13 | 5.0 | 3100 |
| 74 | PM J06579+6219 | M5.0 | - | 2021-02-24.600 | 300sx18 | 4.0 | 3000 |
| 75 | PM J07364+0704 | M5.0 | 13.24 | 2020-12-02.970 | 300sx16 | 5.5 | 3000 |
| 76 | PM J09449-1220 | M5.0 | 13.65 | 2020-11-27.914 | 300sx15 | 4.0 | 3200 |
| 77 | PM J12142+0037 | M5.0 | - | 2021-02-23.879 | 300sx18 | 4.0 | 3100 |
| 78 | PM J13005+0541 | M5.0 | - | 2021-02-23.972 | 300sx17 | 4.5 | 3100 |
| 79 | PM J20298+0941 | M5.0 | - | 2020-11-28.570 | 400sx12 | 5.0 | 3000 |
| 80 | PM J12332+0901 | M5.5 | 12.47 | 2020-12-29.950 | 300sx11 | 4.0 | 3200 |
| 81 | PM J17338+1655 | M5.5 | 14.38 | 2021-03-25.944 | 300sx18 | 5.5 | 3000 |
| 82 | PM J10564+0700 | M6.0 | 13.51 | 2020-11-27.989 | 300sx12 | 4.0 | 3000 |
| 83 | PM J11055+4331 | M6.5 | 14.45 | 2020-12-31.011 | 400sx9 | 5.5 | 3000 |

Table 2: The derived variability parameters for Hα and Hβ emission lines for the sources of this study, along with the activity strengths ( $\log_{10}(L_{H\alpha}/L_{bol})$ and $\log_{10}(L_{H\beta}/L_{bol})$). The $p$-values are determined from the $\chi^2$ minimisation of EW light curves. The sources which are characterize as variable are marked with ($\star$).

| Source ID | Source name | emission line | Median Hα EW Hβ EW | Minimum Hα EW Hβ EW | Maximum Hα EW Hβ EW | Δ Hα EW Hβ EW | RMS Hα EW Hβ EW | Mean $\log_{10}(L_{H\alpha}/L_{bol})$ $\log_{10}(L_{H\beta}/L_{bol})$ | P-value Hα Hβ |
|---|---|---|---|---|---|---|---|---|---|
| 1 | PM J03332+4615S⋆ | Hα | -2.333 ± 0.065 | -1.717 ± 0.062 | -2.492 ± 0.061 | 0.775 ± 0.087 | 0.232 ± 0.022 | -3.883 | 0.0000 |
| | | Hβ | -1.372 ± 0.085 | -0.413 ± 0.091 | -1.590 ± 0.086 | 1.177 ± 0.125 | 0.349 ± 0.031 | -4.199 | 0.0000 |
| 2 | PM J03416+5513 | Hα | -1.688 ± 0.047 | -1.587 ± 0.045 | -1.775 ± 0.052 | 0.188 ± 0.068 | 0.051 ± 0.012 | -3.984 | 0.2298 |
| | | Hβ | -1.818 ± 0.085 | -1.690 ± 0.076 | -1.947 ± 0.087 | 0.258 ± 0.116 | 0.080 ± 0.020 | -3.981 | 0.4134 |
| 3 | PM J07151+1555⋆ | Hα | -2.094 ± 0.052 | -1.372 ± 0.046 | -2.246 ± 0.055 | 0.874 ± 0.072 | 0.183 ± 0.012 | -3.854 | 0.0000 |
| | | Hβ | -1.755 ± 0.076 | -1.525 ± 0.077 | -1.942 ± 0.081 | 0.417 ± 0.111 | 0.110 ± 0.019 | -3.905 | 0.0062 |
| 4 | PM J23083-1524⋆ | Hα | -1.698 ± 0.110 | -1.298 ± 0.061 | -2.010 ± 0.117 | 0.711 ± 0.132 | 0.220 ± 0.025 | -3.980 | 0.0000 |
| | | Hβ | - | - | - | - | - | - | - |
| 5 | PM J03322+4914S⋆ | Hα | -1.637 ± 0.059 | -1.249 ± 0.056 | -2.311 ± 0.066 | 1.062 ± 0.087 | 0.346 ± 0.015 | -3.960 | 0.0000 |
| | | Hβ | -2.431 ± 0.121 | -1.486 ± 0.111 | -4.612 ± 0.141 | 3.127 ± 0.179 | 0.979 ± 0.032 | -3.766 | 0.0000 |
| 6 | PM J04595+0147⋆ | Hα | -1.516 ± 0.039 | -1.421 ± 0.037 | -1.677 ± 0.043 | 0.256 ± 0.057 | 0.061 ± 0.010 | -4.033 | 0.0012 |
| | | Hβ | -1.673 ± 0.067 | -1.574 ± 0.065 | -1.916 ± 0.068 | 0.342 ± 0.094 | 0.091 ± 0.016 | -4.030 | 0.0083 |
| 7 | PM J10143+2104⋆ | Hα | -1.817 ± 0.044 | -1.499 ± 0.041 | -2.033 ± 0.048 | 0.533 ± 0.063 | 0.219 ± 0.013 | -3.973 | 0.0000 |
| | | Hβ | -2.239 ± 0.078 | -1.560 ± 0.066 | -2.787 ± 0.082 | 1.226 ± 0.105 | 0.456 ± 0.022 | -3.940 | 0.0000 |
| 8 | PM J19026+3231⋆ | Hα | -2.532 ± 0.064 | -1.988 ± 0.057 | -2.918 ± 0.069 | 0.930 ± 0.090 | 0.290 ± 0.016 | -3.815 | 0.0000 |
| | | Hβ | - | - | - | - | - | - | - |
| 9 | PM J23060+6355 | Hα | -1.552 ± 0.045 | -1.518 ± 0.045 | -1.619 ± 0.043 | 0.101 ± 0.062 | 0.029 ± 0.013 | -4.057 | 0.9234 |
| | | Hβ | -1.902 ± 0.091 | -1.629 ± 0.089 | -2.042 ± 0.085 | 0.413 ± 0.123 | 0.100 ± 0.027 | -4.046 | 0.1749 |
| 10 | PM J06310+5002⋆ | Hα | -2.112 ± 0.053 | -2.032 ± 0.049 | -2.415 ± 0.056 | 0.382 ± 0.075 | 0.096 ± 0.013 | -3.907 | 0.0000 |
| | | Hβ | -2.541 ± 0.086 | -2.364 ± 0.086 | -3.426 ± 0.102 | 1.062 ± 0.133 | 0.255 ± 0.023 | -3.884 | 0.0000 |
| 11 | PM J08317+0545⋆ | Hα | -2.855 ± 0.096 | -2.583 ± 0.088 | -3.225 ± 0.112 | 0.642 ± 0.143 | 0.173 ± 0.026 | -3.781 | 0.0000 |
| | | Hβ | -2.799 ± 0.221 | -2.322 ± 0.248 | -3.882 ± 0.259 | 1.560 ± 0.359 | 0.484 ± 0.065 | -3.823 | 0.0000 |
| 12 | PM J09193+6203 | Hα | -2.164 ± 0.066 | -2.067 ± 0.066 | -2.213 ± 0.069 | 0.146 ± 0.096 | 0.041 ± 0.017 | -3.865 | 0.9796 |
| | | Hβ | -2.816 ± 0.178 | -1.923 ± 0.186 | -3.238 ± 0.217 | 1.315 ± 0.286 | 0.382 ± 0.052 | -3.776 | 0.0000 |
| 13 | PM J12576+3513E⋆ | Hα | -1.965 ± 0.051 | -1.842 ± 0.047 | -2.068 ± 0.063 | 0.226 ± 0.079 | 0.066 ± 0.014 | -3.928 | 0.0479 |
| | | Hβ | -2.217 ± 0.085 | -1.889 ± 0.074 | -2.405 ± 0.090 | 0.517 ± 0.117 | 0.164 ± 0.028 | -3.923 | 0.0000 |
| 14 | PM J15238+5609⋆ | Hα | -1.726 ± 0.051 | -1.567 ± 0.049 | -1.793 ± 0.051 | 0.226 ± 0.071 | 0.068 ± 0.012 | -3.994 | 0.0112 |
| | | Hβ | - | - | - | - | - | - | - |
| 15 | PM J15581+4927⋆ | Hα | -2.606 ± 0.068 | -2.352 ± 0.087 | -2.733 ± 0.080 | 0.381 ± 0.119 | 0.125 ± 0.032 | -3.897 | 0.0162 |
| | | Hβ | -2.743 ± 0.139 | -2.208 ± 0.270 | -4.415 ± 0.316 | 2.207 ± 0.416 | 0.639 ± 0.110 | -3.998 | 0.0000 |
| 16 | PM J04376-0229 | Hα | -2.994 ± 0.068 | -2.936 ± 0.067 | -3.137 ± 0.072 | 0.201 ± 0.098 | 0.060 ± 0.020 | -3.720 | 0.6793 |
| | | Hβ | -2.911 ± 0.160 | -2.695 ± 0.161 | -3.437 ± 0.120 | 0.743 ± 0.201 | 0.185 ± 0.035 | -3.753 | 0.0010 |
| 17 | PM J00428+3532 | Hα | -2.545 ± 0.061 | -2.451 ± 0.061 | -2.711 ± 0.065 | 0.260 ± 0.089 | 0.078 ± 0.018 | -3.878 | 0.0655 |
| | | Hβ | -3.116 ± 0.128 | -2.968 ± 0.116 | -3.317 ± 0.120 | 0.349 ± 0.167 | 0.103 ± 0.035 | -3.911 | 0.6763 |
| 18 | PM J05402+1239 | Hα | -2.215 ± 0.054 | -2.153 ± 0.053 | -2.324 ± 0.055 | 0.171 ± 0.077 | 0.053 ± 0.013 | -3.931 | 0.4400 |
| | | Hβ | -2.309 ± 0.080 | -2.046 ± 0.084 | -2.429 ± 0.088 | 0.383 ± 0.122 | 0.082 ± 0.021 | -4.028 | 0.4803 |
| 19 | PM J06262+2349⋆ | Hα | -1.520 ± 0.057 | -1.346 ± 0.059 | -1.649 ± 0.060 | 0.303 ± 0.084 | 0.079 ± 0.016 | -4.039 | 0.0232 |
| | | Hβ | -1.804 ± 0.206 | -1.452 ± 0.171 | -2.538 ± 0.237 | 1.086 ± 0.292 | 0.297 ± 0.054 | -3.976 | 0.0018 |
| 20 | PM J07295+3556⋆ | Hα | -2.892 ± 0.070 | -2.733 ± 0.067 | -3.249 ± 0.078 | 0.515 ± 0.102 | 0.122 ± 0.018 | -3.775 | 0.0000 |
| | | Hβ | -3.381 ± 0.133 | -3.103 ± 0.123 | -4.253 ± 0.151 | 1.149 ± 0.195 | 0.268 ± 0.034 | -3.766 | 0.0000 |
| 21 | PM J13007+1222 | Hα | -2.063 ± 0.050 | -1.969 ± 0.048 | -2.132 ± 0.051 | 0.164 ± 0.070 | 0.037 ± 0.012 | -3.986 | 0.8947 |
| | | Hβ | -2.192 ± 0.074 | -2.088 ± 0.075 | -2.460 ± 0.075 | 0.371 ± 0.106 | 0.086 ± 0.018 | -4.090 | 0.1217 |
| 22 | PM J15416+1828⋆ | Hα | -2.218 ± 0.065 | -2.037 ± 0.058 | -2.311 ± 0.065 | 0.274 ± 0.087 | 0.088 ± 0.018 | -3.965 | 0.0086 |
| | | Hβ | -2.475 ± 0.115 | -2.333 ± 0.117 | -2.831 ± 0.128 | 0.498 ± 0.173 | 0.132 ± 0.036 | -4.054 | 0.2102 |
| 23 | PM J16220+2250 | Hα | -3.012 ± 0.075 | -2.866 ± 0.076 | -3.156 ± 0.079 | 0.290 ± 0.109 | 0.082 ± 0.019 | -3.761 | 0.2604 |
| | | Hβ | -3.268 ± 0.130 | -2.946 ± 0.123 | -3.698 ± 0.139 | 0.751 ± 0.185 | 0.181 ± 0.031 | -3.781 | 0.0051 |
| 24 | PM J22387-2037 | Hα | -2.269 ± 0.061 | -2.156 ± 0.056 | -2.357 ± 0.063 | 0.202 ± 0.084 | 0.065 ± 0.015 | -3.869 | 0.2155 |
| | | Hβ | -2.660 ± 0.118 | -2.302 ± 0.155 | -3.125 ± 0.196 | 0.823 ± 0.250 | 0.190 ± 0.040 | -3.847 | 0.0360 |
| 25 | PM J04284+1741⋆ | Hα | -2.976 ± 0.079 | -2.775 ± 0.076 | -3.172 ± 0.083 | 0.398 ± 0.113 | 0.107 ± 0.019 | -3.859 | 0.0103 |
| | | Hβ | -3.296 ± 0.142 | -2.881 ± 0.150 | -4.188 ± 0.171 | 1.307 ± 0.228 | 0.370 ± 0.039 | -3.976 | 0.0000 |
| 26 | PM J06212+4414 | Hα | -2.854 ± 0.076 | -2.762 ± 0.082 | -2.936 ± 0.074 | 0.174 ± 0.110 | 0.055 ± 0.027 | -3.841 | 0.8049 |
| | | Hβ | -3.188 ± 0.160 | -2.923 ± 0.180 | -3.517 ± 0.162 | 0.594 ± 0.242 | 0.223 ± 0.062 | -3.917 | 0.0634 |
| 27 | PM J11201-1029⋆ | Hα | -2.033 ± 0.059 | -1.841 ± 0.054 | -2.206 ± 0.062 | 0.365 ± 0.082 | 0.111 ± 0.014 | -3.976 | 0.0000 |
| | | Hβ | -2.254 ± 0.104 | -1.899 ± 0.110 | -2.733 ± 0.108 | 0.834 ± 0.154 | 0.223 ± 0.027 | -4.045 | 0.0000 |
| 28 | PM J13518+1247⋆ | Hα | -2.118 ± 0.062 | -1.771 ± 0.091 | -2.248 ± 0.072 | 0.478 ± 0.115 | 0.112 ± 0.020 | -3.997 | 0.0071 |
| | | Hβ | -2.680 ± 0.132 | -1.915 ± 0.152 | -3.277 ± 0.153 | 1.363 ± 0.216 | 0.327 ± 0.037 | -4.059 | 0.0000 |
| 29 | PM J15218+2058⋆ | Hα | -2.615 ± 0.060 | -2.383 ± 0.081 | -2.771 ± 0.097 | 0.388 ± 0.126 | 0.099 ± 0.018 | -3.866 | 0.0351 |
| | | Hβ | -2.864 ± 0.216 | -2.430 ± 0.182 | -3.331 ± 0.213 | 0.901 ± 0.280 | 0.244 ± 0.039 | -3.943 | 0.0000 |
| 30 | PM J16170+5516 | Hα | -2.513 ± 0.064 | -2.344 ± 0.077 | -2.628 ± 0.066 | 0.284 ± 0.101 | 0.062 ± 0.019 | -3.900 | 0.7030 |
| | | Hβ | -2.909 ± 0.096 | -2.533 ± 0.140 | -3.380 ± 0.176 | 0.847 ± 0.224 | 0.214 ± 0.039 | -3.974 | 0.0020 |
| 31 | PM J06596+0545 | Hα | -1.775 ± 0.062 | -1.675 ± 0.061 | -1.858 ± 0.062 | 0.182 ± 0.087 | 0.065 ± 0.015 | -4.062 | 0.2529 |
| | | Hβ | -2.069 ± 0.120 | -1.767 ± 0.123 | -2.424 ± 0.118 | 0.657 ± 0.170 | 0.141 ± 0.030 | -4.139 | 0.1106 |
| 32 | PM J09177+4612⋆ | Hα | -3.899 ± 0.085 | -3.674 ± 0.081 | -4.093 ± 0.089 | 0.419 ± 0.120 | 0.117 ± 0.019 | -3.693 | 0.0049 |
| | | Hβ | -4.515 ± 0.134 | -3.989 ± 0.124 | -4.974 ± 0.137 | 0.986 ± 0.185 | 0.258 ± 0.030 | -3.744 | 0.0000 |
| 33 | PM J10043+5023 | Hα | -3.600 ± 0.088 | -3.475 ± 0.083 | -3.788 ± 0.085 | 0.313 ± 0.119 | 0.077 ± 0.020 | -3.739 | 0.5912 |
| | | Hβ | -3.528 ± 0.121 | -3.322 ± 0.133 | -3.768 ± 0.117 | 0.446 ± 0.177 | 0.118 ± 0.030 | -3.874 | 0.4600 |
| 34 | PM J11519+0731 | Hα | -3.009 ± 0.083 | -2.810 ± 0.085 | -3.177 ± 0.084 | 0.367 ± 0.120 | 0.096 ± 0.023 | -3.858 | 0.1592 |
| | | Hβ | -3.051 ± 0.150 | -2.805 ± 0.177 | -3.617 ± 0.142 | 0.812 ± 0.227 | 0.221 ± 0.042 | -4.023 | 0.0063 |
| 35 | PM J15557+6840 | Hα | -2.355 ± 0.076 | -2.201 ± 0.074 | -2.523 ± 0.075 | 0.322 ± 0.105 | 0.092 ± 0.022 | -3.907 | 0.0708 |
| | | Hβ | -2.552 ± 0.157 | -2.104 ± 0.157 | -2.662 ± 0.163 | 0.558 ± 0.226 | 0.159 ± 0.048 | -3.996 | 0.3764 |
| 36 | PM J04333+2359⋆ | Hα | -3.156 ± 0.086 | -2.333 ± 0.072 | -3.511 ± 0.094 | 1.178 ± 0.118 | 0.329 ± 0.020 | -3.846 | 0.0000 |
| | | Hβ | -3.518 ± 0.155 | -2.772 ± 0.146 | -4.090 ± 0.158 | 1.319 ± 0.215 | 0.358 ± 0.038 | -3.948 | 0.0000 |
| 37 | PM J05091+1527⋆ | Hα | -3.211 ± 0.122 | -2.940 ± 0.155 | -3.635 ± 0.154 | 0.695 ± 0.219 | 0.199 ± 0.037 | -3.829 | 0.0150 |
| | | Hβ | - | - | - | - | - | - | - |

Table 2: continues...

| Source | Source | emission | Median | Minimum | Maximum | Δ | RMS | Mean | P-value |
|---|---|---|---|---|---|---|---|---|---|
| ID | name | line | Hα EW | Hα EW | Hα EW | Hα EW | Hα EW | $\log_{10}(L_{H\alpha}/L_{bol})$ | Hα |
| | | | Hβ EW | Hβ EW | Hβ EW | Hβ EW | Hβ EW | $\log_{10}(L_{H\beta}/L_{bol})$ | Hβ |
| 38 | PM J05337+0156 | Hα | -6.394 ± 0.134 | -6.182 ± 0.130 | -6.568 ± 0.136 | 0.386 ± 0.189 | 0.103 ± 0.038 | -3.510 | 0.8028 |
| | | Hβ | -6.956 ± 0.191 | -6.580 ± 0.189 | -7.451 ± 0.196 | 0.871 ± 0.272 | 0.208 ± 0.055 | -3.628 | 0.2125 |
| 39 | PM J05547+1055$^\star$ | Hα | -4.045 ± 0.099 | -3.692 ± 0.096 | -4.405 ± 0.103 | 0.713 ± 0.141 | 0.210 ± 0.024 | -3.739 | 0.0000 |
| | | Hβ | -4.459 ± 0.199 | -3.945 ± 0.196 | -5.078 ± 0.204 | 1.132 ± 0.282 | 0.238 ± 0.047 | -3.877 | 0.0594 |
| 40 | PM J07319+3613S$^\star$ | Hα | -1.871 ± 0.065 | -1.382 ± 0.055 | -2.020 ± 0.065 | 0.639 ± 0.085 | 0.187 ± 0.014 | -4.136 | 0.0000 |
| | | Hβ | -2.072 ± 0.131 | -1.146 ± 0.093 | -2.676 ± 0.127 | 1.530 ± 0.158 | 0.434 ± 0.028 | -4.311 | 0.0000 |
| 41 | PM J07349+1445 | Hα | -2.451 ± 0.071 | -2.355 ± 0.070 | -2.574 ± 0.074 | 0.219 ± 0.102 | 0.051 ± 0.017 | -3.967 | 0.9333 |
| | | Hβ | - | - | - | - | - | - | - |
| 42 | PM J11529+3554$^\star$ | Hα | -4.697 ± 0.202 | -3.708 ± 0.310 | -5.760 ± 0.280 | 2.052 ± 0.417 | 0.593 ± 0.094 | -3.628 | 0.0000 |
| | | Hβ | -4.100 ± 1.131 | -3.013 ± 0.937 | -6.610 ± 1.401 | 3.598 ± 1.686 | 1.080 ± 0.415 | -3.805 | 0.3939 |
| 43 | PM J12355+2439$^\star$ | Hα | -2.467 ± 0.096 | -2.297 ± 0.098 | -2.779 ± 0.102 | 0.482 ± 0.141 | 0.132 ± 0.032 | -3.913 | 0.0263 |
| | | Hβ | -3.036 ± 0.249 | -2.703 ± 0.213 | -3.996 ± 0.284 | 1.292 ± 0.355 | 0.402 ± 0.101 | -3.952 | 0.0074 |
| 44 | PM J13352+1714$^\star$ | Hα | -2.696 ± 0.083 | -2.417 ± 0.120 | -2.917 ± 0.139 | 0.500 ± 0.184 | 0.170 ± 0.041 | - | 0.0082 |
| | | Hβ | -3.025 ± 0.175 | -2.460 ± 0.229 | -3.773 ± 0.302 | 1.313 ± 0.378 | 0.414 ± 0.103 | - | 0.0107 |
| 45 | PM J14137+4618 | Hα | -4.520 ± 0.119 | -4.313 ± 0.129 | -4.774 ± 0.122 | 0.461 ± 0.178 | 0.148 ± 0.044 | -3.768 | 0.1292 |
| | | Hβ | -4.966 ± 0.342 | -3.373 ± 0.410 | -6.525 ± 0.282 | 3.152 ± 0.498 | 0.906 ± 0.123 | -3.992 | 0.0000 |
| 46 | PM J04238+1455 | Hα | -5.064 ± 0.360 | -4.235 ± 0.292 | -5.419 ± 0.294 | 1.184 ± 0.414 | 0.367 ± 0.102 | -3.711 | 0.0919 |
| | | Hβ | -9.320 ± 1.001 | -3.474 ± 0.545 | -15.323 ± 1.809 | 11.849 ± 1.890 | 4.045 ± 0.438 | -3.672 | 0.0000 |
| 47 | PM J09302+2630$^\star$ | Hα | -3.100 ± 0.095 | -2.765 ± 0.098 | -3.470 ± 0.104 | 0.705 ± 0.143 | 0.189 ± 0.024 | -3.893 | 0.0000 |
| | | Hβ | - | - | - | - | - | - | - |
| 48 | PM J09557+3521$^\star$ | Hα | -2.956 ± 0.096 | -2.610 ± 0.104 | -3.316 ± 0.102 | 0.706 ± 0.146 | 0.193 ± 0.027 | -3.915 | 0.0000 |
| | | Hβ | - | - | - | - | - | - | - |
| 49 | PM J12485+4933 | Hα | -5.196 ± 0.124 | -4.989 ± 0.121 | -5.444 ± 0.124 | 0.455 ± 0.173 | 0.142 ± 0.033 | -3.641 | 0.1323 |
| | | Hβ | -6.051 ± 0.206 | -5.407 ± 0.193 | -6.749 ± 0.213 | 1.342 ± 0.288 | 0.368 ± 0.054 | -3.774 | 0.0000 |
| 50 | PM J12490+6606$^\star$ | Hα | -1.038 ± 0.052 | -0.968 ± 0.050 | -1.302 ± 0.050 | 0.334 ± 0.071 | 0.078 ± 0.012 | -4.387 | 0.0007 |
| | | Hβ | -0.960 ± 0.095 | -0.802 ± 0.092 | -1.152 ± 0.104 | 0.350 ± 0.138 | 0.110 ± 0.024 | -4.662 | 0.1525 |
| 51 | PM J13417+5815$^\star$ | Hα | -2.323 ± 0.083 | -1.813 ± 0.072 | -3.243 ± 0.095 | 1.430 ± 0.119 | 0.403 ± 0.021 | -4.008 | 0.0000 |
| | | Hβ | -2.575 ± 0.208 | -1.788 ± 0.179 | -4.175 ± 0.217 | 2.387 ± 0.282 | 0.585 ± 0.049 | -4.164 | 0.0000 |
| 52 | PM J16591+2058$^\star$ | Hα | -3.206 ± 0.091 | -3.007 ± 0.088 | -3.626 ± 0.101 | 0.619 ± 0.134 | 0.169 ± 0.023 | -3.880 | 0.0000 |
| | | Hβ | -3.311 ± 0.161 | -2.753 ± 0.143 | -4.216 ± 0.172 | 1.463 ± 0.224 | 0.424 ± 0.041 | -4.091 | 0.0000 |
| 53 | PM J00325+0729 | Hα | -5.958 ± 0.147 | -5.796 ± 0.144 | -6.302 ± 0.160 | 0.506 ± 0.215 | 0.153 ± 0.046 | -3.629 | 0.3676 |
| | | Hβ | -5.477 ± 0.222 | -5.111 ± 0.226 | -6.179 ± 0.255 | 1.068 ± 0.341 | 0.367 ± 0.089 | -3.903 | 0.0113 |
| 54 | PM J01593+5831 | Hα | -6.089 ± 0.146 | -5.796 ± 0.144 | -6.277 ± 0.153 | 0.480 ± 0.210 | 0.161 ± 0.041 | -3.700 | 0.2252 |
| | | Hβ | -6.800 ± 0.240 | -6.022 ± 0.225 | -7.646 ± 0.243 | 1.624 ± 0.331 | 0.522 ± 0.065 | -3.963 | 0.0000 |
| 55 | PM J02088+4926$^\star$ | Hα | -7.213 ± 0.157 | -6.340 ± 0.144 | -7.947 ± 0.172 | 1.607 ± 0.225 | 0.569 ± 0.044 | -3.534 | 0.0000 |
| | | Hβ | -9.140 ± 0.273 | -7.573 ± 0.237 | -10.534 ± 0.308 | 2.961 ± 0.388 | 0.986 ± 0.075 | -3.661 | 0.0000 |
| 56 | PM J05062+0439$^\star$ | Hα | -7.327 ± 0.183 | -6.835 ± 0.175 | -7.682 ± 0.189 | 0.847 ± 0.258 | 0.227 ± 0.044 | -3.662 | 0.0422 |
| | | Hβ | -8.301 ± 0.306 | -7.359 ± 0.291 | -9.795 ± 0.323 | 2.436 ± 0.434 | 0.504 ± 0.076 | -3.957 | 0.0001 |
| 57 | PM J06000+0242$^\star$ | Hα | -2.782 ± 0.085 | -2.618 ± 0.083 | -3.119 ± 0.088 | 0.501 ± 0.121 | 0.142 ± 0.021 | -4.042 | 0.0001 |
| | | Hβ | -2.928 ± 0.147 | -2.368 ± 0.133 | -3.680 ± 0.149 | 1.312 ± 0.200 | 0.348 ± 0.035 | -4.351 | 0.0000 |
| 58 | PM J07033+3441$^\star$ | Hα | -5.124 ± 0.137 | -4.467 ± 0.121 | -5.559 ± 0.143 | 1.091 ± 0.188 | 0.301 ± 0.032 | -3.730 | 0.0000 |
| | | Hβ | -5.389 ± 0.246 | -4.700 ± 0.222 | -7.483 ± 0.275 | 2.782 ± 0.353 | 0.859 ± 0.061 | -3.957 | 0.0000 |
| 59 | PM J07100+3831 | Hα | -1.850 ± 0.091 | -1.682 ± 0.087 | -2.121 ± 0.096 | 0.439 ± 0.130 | 0.109 ± 0.022 | -4.296 | 0.0719 |
| | | Hβ | -1.518 ± 0.144 | -1.159 ± 0.162 | -2.295 ± 0.158 | 1.135 ± 0.226 | 0.273 ± 0.038 | -4.760 | 0.0000 |
| 60 | PM J09161+0153$^\star$ | Hα | -4.709 ± 0.132 | -4.443 ± 0.132 | -5.361 ± 0.146 | 0.918 ± 0.197 | 0.239 ± 0.035 | -3.751 | 0.0000 |
| | | Hβ | -5.232 ± 0.314 | -4.748 ± 0.236 | -5.850 ± 0.246 | 1.102 ± 0.341 | 0.403 ± 0.070 | -3.968 | 0.0013 |
| 61 | PM J10357+0215$^\star$ | Hα | -3.423 ± 0.160 | -2.978 ± 0.204 | -4.019 ± 0.202 | 1.040 ± 0.287 | 0.335 ± 0.096 | -3.791 | 0.0067 |
| | | Hβ | -3.811 ± 0.419 | -3.313 ± 0.806 | -7.983 ± 1.511 | 4.670 ± 1.713 | 1.738 ± 0.635 | -3.840 | 0.0061 |
| 62 | PM J10360+0507$^\star$ | Hα | -5.604 ± 0.140 | -5.435 ± 0.134 | -6.462 ± 0.158 | 1.027 ± 0.208 | 0.262 ± 0.037 | -3.670 | 0.0000 |
| | | Hβ | -6.182 ± 0.247 | -5.458 ± 0.249 | -8.427 ± 0.313 | 2.969 ± 0.400 | 0.808 ± 0.067 | -3.880 | 0.0000 |
| 63 | PM J11033+1337$^\star$ | Hα | -3.094 ± 0.102 | -2.961 ± 0.102 | -3.572 ± 0.111 | 0.612 ± 0.151 | 0.141 ± 0.026 | -3.909 | 0.0271 |
| | | Hβ | - | - | - | - | - | - | - |
| 64 | PM J11118+3332S | Hα | -5.423 ± 0.126 | -5.086 ± 0.178 | -5.696 ± 0.132 | 0.611 ± 0.222 | 0.177 ± 0.053 | -3.682 | 0.1206 |
| | | Hβ | -6.126 ± 0.204 | -4.150 ± 0.739 | -6.964 ± 0.714 | 2.814 ± 1.028 | 0.801 ± 0.195 | -3.908 | 0.0000 |
| 65 | PM J12156+5239 | Hα | -5.364 ± 0.124 | -5.219 ± 0.122 | -5.496 ± 0.127 | 0.277 ± 0.176 | 0.073 ± 0.030 | -3.731 | 0.9915 |
| | | Hβ | -6.213 ± 0.193 | -5.962 ± 0.190 | -7.080 ± 0.214 | 1.117 ± 0.286 | 0.245 ± 0.050 | -3.960 | 0.0873 |
| 66 | PM J13536+7737$^\star$ | Hα | -3.485 ± 0.121 | -3.226 ± 0.110 | -5.818 ± 0.150 | 2.593 ± 0.186 | 0.574 ± 0.035 | -3.926 | 0.0000 |
| | | Hβ | -3.837 ± 0.401 | -2.199 ± 0.430 | -14.037 ± 0.576 | 11.838 ± 0.718 | 2.654 ± 0.130 | -4.160 | 0.0000 |
| 67 | PM J14165-0725 | Hα | -3.559 ± 0.143 | -3.401 ± 0.141 | -3.742 ± 0.132 | 0.341 ± 0.194 | 0.120 ± 0.046 | -3.890 | 0.5877 |
| | | Hβ | -5.528 ± 0.573 | -4.366 ± 0.569 | -6.791 ± 0.498 | 2.426 ± 0.756 | 0.833 ± 0.168 | -3.988 | 0.0007 |
| 68 | PM J15126+4543$^\star$ | Hα | -4.034 ± 0.179 | -3.706 ± 0.172 | -4.725 ± 0.173 | 1.019 ± 0.244 | 0.302 ± 0.042 | -3.840 | 0.0000 |
| | | Hβ | -4.759 ± 0.664 | -3.784 ± 0.263 | -7.641 ± 0.695 | 3.858 ± 0.743 | 1.023 ± 0.154 | -4.054 | 0.0000 |
| 69 | PM J05243-1601$^\star$ | Hα | -10.500 ± 0.256 | -9.080 ± 0.233 | -10.776 ± 0.272 | 1.696 ± 0.359 | 0.549 ± 0.069 | -3.502 | 0.0000 |
| | | Hβ | -12.443 ± 0.486 | -9.432 ± 0.446 | -14.962 ± 0.520 | 5.529 ± 0.685 | 1.561 ± 0.130 | -3.762 | 0.0000 |
| 70 | PM J13317+2916 | Hα | -9.108 ± 0.201 | -8.917 ± 0.195 | -9.493 ± 0.207 | 0.576 ± 0.285 | 0.192 ± 0.054 | -3.565 | 0.4687 |
| | | Hβ | -9.005 ± 0.239 | -8.696 ± 0.241 | -10.964 ± 0.280 | 2.268 ± 0.369 | 0.666 ± 0.070 | -3.910 | 0.0000 |
| 71 | PM J17199+2630W | Hα | -2.153 ± 0.080 | -2.078 ± 0.078 | -2.195 ± 0.082 | 0.117 ± 0.113 | 0.036 ± 0.028 | -4.188 | 0.9852 |
| | | Hβ | -2.019 ± 0.172 | -1.489 ± 0.222 | -2.463 ± 0.177 | 0.974 ± 0.284 | 0.260 ± 0.068 | -4.567 | 0.0284 |
| 72 | PM J01033+6221 | Hα | -14.374 ± 0.327 | -13.836 ± 0.328 | -15.019 ± 0.347 | 1.183 ± 0.477 | 0.369 ± 0.096 | -3.424 | 0.2004 |
| | | Hβ | -21.756 ± 0.697 | -19.777 ± 0.649 | -27.742 ± 0.804 | 7.965 ± 1.033 | 2.373 ± 0.215 | -3.626 | 0.0000 |
| 73 | PM J02002+1303 | Hα | -2.053 ± 0.104 | -1.912 ± 0.095 | -2.322 ± 0.106 | 0.410 ± 0.143 | 0.125 ± 0.029 | -4.198 | 0.0742 |
| | | Hβ | -1.326 ± 0.215 | -0.864 ± 0.203 | -1.888 ± 0.194 | 1.023 ± 0.281 | 0.306 ± 0.058 | -4.734 | 0.0027 |
| 74 | PM J06579+6219$^\star$ | Hα | -2.558 ± 0.127 | -2.225 ± 0.125 | -3.362 ± 0.135 | 1.137 ± 0.184 | 0.288 ± 0.032 | -4.180 | 0.0000 |
| | | Hβ | -2.656 ± 0.410 | -1.542 ± 0.440 | -4.644 ± 0.330 | 3.102 ± 0.550 | 0.808 ± 0.094 | -4.577 | 0.0000 |
| 75 | PM J07364+0704$^\star$ | Hα | -5.606 ± 0.174 | -5.010 ± 0.159 | -5.863 ± 0.174 | 0.853 ± 0.236 | 0.255 ± 0.043 | -3.890 | 0.0011 |
| | | Hβ | -6.995 ± 0.389 | -5.897 ± 0.345 | -9.587 ± 0.462 | 3.689 ± 0.577 | 1.152 ± 0.102 | -4.217 | 0.0000 |
| 76 | PM J09449-1220$^\star$ | Hα | -12.969 ± 0.313 | -12.313 ± 0.302 | -16.936 ± 0.389 | 4.623 ± 0.492 | 1.432 ± 0.095 | -3.589 | 0.0000 |
| | | Hβ | -14.558 ± 0.450 | -12.798 ± 0.555 | -34.008 ± 0.857 | 21.210 ± 1.021 | 6.434 ± 0.191 | -3.985 | 0.0000 |

Table 2: continues...

| Source ID | Source name | emission line | Median Hα EW Hβ EW | Minimum Hα EW Hβ EW | Maximum Hα EW Hβ EW | Δ Hα EW Hβ EW | RMS Hα EW Hβ EW | Mean $\log_{10}(L_{H\alpha}/L_{bol})$ $\log_{10}(L_{H\beta}/L_{bol})$ | P-value Hα Hβ |
|---|---|---|---|---|---|---|---|---|---|
| 77 | PM J12142+0037⋆ | Hα | -7.256 ± 0.233 | -6.326 ± 0.214 | -8.113 ± 0.241 | 1.787 ± 0.322 | 0.492 ± 0.057 | -3.808 | 0.0000 |
| | | Hβ | -12.128 ± 0.765 | -6.575 ± 0.681 | -14.916 ± 0.666 | 8.341 ± 0.952 | 2.693 ± 0.193 | -4.087 | 0.0000 |
| 78 | PM J13005+0541⋆ | Hα | -7.589 ± 0.208 | -7.055 ± 0.195 | -9.026 ± 0.232 | 1.971 ± 0.303 | 0.502 ± 0.056 | -3.646 | 0.0000 |
| | | Hβ | -9.765 ± 0.518 | -8.155 ± 0.482 | -14.109 ± 0.660 | 5.954 ± 0.817 | 1.433 ± 0.147 | -3.889 | 0.0000 |
| 79 | PM J20298+0941⋆ | Hα | -5.622 ± 0.158 | -5.053 ± 0.171 | -8.264 ± 0.222 | 3.212 ± 0.280 | 0.870 ± 0.062 | -3.813 | 0.0000 |
| | | Hβ | -7.182 ± 0.336 | -5.312 ± 0.699 | -17.770 ± 0.861 | 12.458 ± 1.109 | 3.106 ± 0.245 | -4.076 | 0.0000 |
| 80 | PM J12332+0901⋆ | Hα | -6.706 ± 0.210 | -6.411 ± 0.233 | -7.350 ± 0.232 | 0.939 ± 0.329 | 0.322 ± 0.072 | -3.872 | 0.0123 |
| | | Hβ | -9.305 ± 0.355 | -8.079 ± 0.329 | -13.386 ± 0.791 | 5.307 ± 0.856 | 1.433 ± 0.201 | -4.216 | 0.0000 |
| 81 | PM J17338+1655⋆ | Hα | -16.011 ± 0.394 | -15.034 ± 0.376 | -17.078 ± 0.419 | 2.044 ± 0.563 | 0.580 ± 0.096 | -3.526 | 0.0019 |
| | | Hβ | -15.474 ± 0.780 | -12.478 ± 0.651 | -18.510 ± 0.799 | 6.032 ± 1.030 | 1.537 ± 0.182 | -4.066 | 0.0000 |
| 82 | PM J10564+0700⋆ | Hα | -9.604 ± 0.303 | -7.968 ± 0.276 | -10.721 ± 0.322 | 2.753 ± 0.425 | 0.726 ± 0.090 | -3.746 | 0.0000 |
| | | Hβ | -13.160 ± 0.499 | -9.466 ± 0.433 | -18.432 ± 0.572 | 8.966 ± 0.717 | 2.485 ± 0.155 | -4.100 | 0.0000 |
| 83 | PM J11055+4331⋆ | Hα | -11.761 ± 0.357 | -9.479 ± 0.288 | -17.546 ± 0.478 | 8.067 ± 0.558 | 2.260 ± 0.147 | -3.850 | 0.0000 |
| | | Hβ | -23.353 ± 1.646 | -13.665 ± 0.782 | -36.401 ± 2.937 | 22.736 ± 3.039 | 6.440 ± 0.806 | -4.258 | 0.0000 |

Table 3: Derived rotation periods and star-spot filling factors of the objects of this study using TESS and Kepler/K2 light curves. The rotation periods from the literature survey are also mentioned with references and remark (if any). The observing details from TESS and Kepler/K2 archives and computed mean values of FLI for H$\alpha$ and H$\beta$ emissions from the spectral time series are also mentioned. The flaring sources (as per FLI criteria) during the spectroscopy observations are marked with ($\star$) in the source-name column. In the third column (mission/year/author) column, the notation 'T' represents TESS sector and a 'K' represents K2 campaign.

| Source ID | Source name | Mission/Year/Author | Exposure time (s) | Rotation period (days) | Rotation Period from literature[b] (days) | Ref.[a] | $T_{spot}$ (K) | Filling factor % | Mean FLI Hα | Mean FLI Hβ |
|---|---|---|---|---|---|---|---|---|---|---|
| 1 | PM J03332+4615S⋆ | T-18/2019/QLP | 1800 | 3.160 | - | - | 3192 | 36 | 10.40 ± 1.72 | 2.65 ± 0.95 |
| 2 | PM J03416+5513⋆ | T-19/2019/SPOC | 120 | 4.641 | 8[1] | 4 | 3145 | 6.2 | 6.97 ± 0.62 | 4.50 ± 0.45 |
| 3 | PM J07151+1555⋆ | T-33/2020/SPOC | 120 | 0.554 | 0.555 | 6 | 3239 | 9.6 | 12.05 ± 1.83 | 4.67 ± 0.42 |
| 4 | PM J23083-1524 | T-42/2021/SPOC | 20 | 0.432 | 0.431 | 6 | 3192 | 8.9 | 6.17 ± 1.25 | - |
| 5 | PM J03322+4914S⋆ | T-18/2019/SPOC | 120 | 5.799 | 5.947 | 9 | 3097 | 5 | 7.09 ± 1.59 | 6.23 ± 2.72 |
| 6 | PM J04595+0147⋆ | T-32/2020/SPOC | 120 | 4.406 | 4.414 | 6 | 3192 | 7.1 | 6.75 ± 0.43 | 4.63 ± 0.50 |
| 7 | PM J10143+2104⋆ | - | - | - | 7.861 | 6 | 3145 | - | 8.00 ± 1.36 | 5.28 ± 1.25 |
| 8 | PM J19026+3231 | T-14/2019/SPOC | 120 | 0.347 | 3.545[2] | 9 | 3097 | 7.6 | 11.91 ± 2.38 | - |
| 9 | PM J23060+6355⋆ | T-24/2020/SPOC | 120 | 2.848 | 2.831 | 5 | 3097 | 11.3 | 6.96 ± 0.66 | 4.33 ± 0.55 |
| 10 | PM J06310+5002⋆ | T-20/2019/SPOC | 120 | 4.966 | 15.25[2] | 9 | 3097 | 2.6 | 8.68 ± 1.04 | 6.32 ± 0.81 |
| 11 | PM J08317+0545⋆ | T-07/2019/SPOC | 120 | 0.595 | 1.4755[2] | 6 | 3145 | 4.6 | 10.06 ± 0.96 | 4.13 ± 1.06 |
| 12 | PM J09193+6203⋆ | T-21/2020/SPOC | 120 | - | 2.992 | 9 | 3048 | 3 | 8.22 ± 0.60 | 4.03 ± 0.74 |
| 13 | PM J12576+3513E⋆ | T-22/2020/SPOC | 120 | 3.355 | 3.170 | 5 | 3048 | 7.7 | 7.95 ± 0.79 | 5.09 ± 0.76 |
| 14 | PM J15238+5609 | T-24/2020/SPOC | 120 | 1.003 | - | - | 3145 | 5 | 7.26 ± 0.64 | - |
| 15 | PM J15581+4927⋆ | T-24/2020/SPOC | 120 | 0.815 | 4.492[2] | 9 | 3048 | 8.5 | 9.17 ± 1.28 | 3.97 ± 0.92 |
| 16 | PM J04376-0229 | T-05/2018/QLP | 1800 | - | 4.890 | 1 | 3048 | - | 11.35 ± 0.65 | 6.48 ± 0.98 |
| 17 | PM J00428+3532⋆ | T-17/2019/SPOC | 120 | 2.174 | 2.170 | 4 | 2998 | 6.4 | 10.02 ± 0.97 | 6.04 ± 0.76 |
| 18 | PM J05402+1239⋆ | T-06/2018/SPOC | 120 | 1.589 | 0.6125[2] | 5 | 3097 | 6.8 | 9.36 ± 0.77 | 6.02 ± 0.71 |
| 19 | PM J06262+2349 | K/2014/K2 | 1800 | 8.059 | 7.890 | 4 | 2998 | 5.8 | 5.20 ± 0.46 | 2.81 ± 0.81 |
| 20 | PM J07295+3556⋆ | T-20/2019/SPOC | 120 | 1.979 | 1.970 | 1 | 3048 | 7.2 | 11.36 ± 1.07 | 7.40 ± 0.60 |
| 21 | PM J13007+1222 | T-23/2020/SPOC | 120 | 2.881 | 2.886 | 6 | 3192 | 9.5 | 8.20 ± 0.57 | 6.15 ± 0.65 |
| 22 | PM J15416+1828⋆ | T-24/2020/TESS-SPOC | 1800 | - | - | - | 3048 | - | 8.39 ± 0.74 | 5.90 ± 0.70 |
| 23 | PM J16220+2250 | T-25/2020/QLP | 1800 | - | - | - | 3097 | 7.2 | 10.78 ± 0.72 | 8.12 ± 0.86 |
| 24 | PM J22387-2037⋆ | T-42/2021/SPOC | 120 | 4.391 | 4.230 | 4 | 3048 | 3.7 | 7.76 ± 0.63 | 4.92 ± 0.82 |
| 25 | PM J04284+1741⋆ | K-13/2017/K2 | 1800 | 2.449 | 2.440 | 4 | 2998 | 10.6 | 10.10 ± 0.91 | 6.08 ± 0.88 |
| 26 | PM J06212+4414 | T-20/2019/SPOC | 120 | 5.848 | 5.728 | 9 | 2998 | 16.1 | 9.33 ± 0.69 | 4.92 ± 0.75 |
| 27 | PM J11201-1029⋆ | T-09/2019/SPOC | 120 | 5.652 | - | - | 2998 | 3.4 | 7.05 ± 0.64 | 4.93 ± 0.84 |
| 28 | PM J13518+1247⋆ | T-23/2020/SPOC | 120 | - | - | - | 3145 | 2.2 | 7.70 ± 1.02 | 5.61 ± 0.95 |
| 29 | PM J15218+2058⋆ | T-24/2020/SPOC | 120 | 3.395 | 3.383 | 5 | 3048 | 3.5 | 9.27 ± 1.24 | 5.85 ± 1.27 |
| 30 | PM J16170+5516⋆ | T-25/2020/SPOC | 120 | 1.975 | - | - | 3048 | 3.7 | 8.79 ± 0.70 | 6.55 ± 0.98 |
| 31 | PM J06596+0545⋆ | T-33/2020/TESS-SPOC | 600 | 10.331 | - | - | 2998 | 2.5 | 5.99 ± 0.46 | 3.94 ± 0.55 |
| 32 | PM J09177+4612⋆ | T-21/2020/SPOC | 120 | 1.016 | 0.56[3] | 4 | 2998 | 7.4 | 13.47 ± 1.16 | 9.70 ± 1.14 |
| 33 | PM J10043+5023⋆ | T-21/2020/SPOC | 120 | 1.315 | 1.313 | 5 | 2998 | 5.9 | 11.19 ± 0.79 | 7.30 ± 0.81 |
| 34 | PM J11519+0731⋆ | T-22/2020/SPOC | 120 | 2.283 | 2.291 | 6 | 2998 | 10.1 | 9.59 ± 0.70 | 6.46 ± 1.23 |
| 35 | PM J15557+6840 | T-40/2021/SPOC | 120 | 3.917 | 3.930 | 8 | 2948 | 4.4 | 7.73 ± 0.56 | 4.43 ± 0.55 |
| 36 | PM J04333+2359⋆ | - | - | - | - | - | 2998 | - | 8.19 ± 0.62 | 6.46 ± 0.69 |
| 37 | PM J05091+1527 | T-32/2020/SPOC | 120 | 2.532 | 2.540 | 10 | 2948 | 1.2 | 7.01 ± 0.92 | - |
| 38 | PM J05337+0156⋆ | T-32/2020/SPOC | 20 | 0.605 | 2.510[4] | 2 | 2948 | 1.3 | 18.46 ± 1.40 | 12.84 ± 1.31 |
| 39 | PM J05547+1055⋆ | T-33/2020/SPOC | 120 | 0.565 | 1.13[2] | 9 | 2998 | 5.5 | 11.63 ± 1.03 | 7.73 ± 1.78 |
| 40 | PM J07319+3613S⋆ | T-20/2019/QLP | 1800 | - | 3.69 | 2 | 2948 | 9.3 | 4.37 ± 0.63 | 3.10 ± 0.88 |
| 41 | PM J07349+1445 | T-07/2019/SPOC | 120 | - | 20.08 | 9 | 2948 | 2.3 | 5.80 ± 0.42 | - |
| 42 | PM J11529+3554 | T-22/2020/SPOC | 120 | 2.690 | 2.69 | 4 | 2896 | 6 | 8.36 ± 1.85 | 1.08 ± 0.53 |
| 43 | PM J12355+2439 | - | - | - | - | - | 2998 | - | 7.79 ± 0.56 | 3.82 ± 0.49 |
| 44 | PM J13352+1714⋆ | T-23/2020/SPOC | 120 | 1.213 | - | - | 3048 | 2.2 | 9.02 ± 1.49 | 4.75 ± 1.50 |
| 45 | PM J14137+4618⋆ | T-23/2020/TESS-SPOC | 1800 | 1.536 | - | - | 2948 | 4.4 | 13.28 ± 1.55 | 5.31 ± 2.45 |
| 46 | PM J04238+1455⋆ | T-32/2020/SPOC | 120 | 0.923 | - | - | 2998 | 1.1 | 5.65 ± 1.18 | 2.52 ± 0.94 |
| 47 | PM J09302+2630 | T-21/2020/SPOC | 120 | 10.517 | 10.68 | 11 | 2948 | 1.3 | 6.36 ± 0.64 | - |
| 48 | PM J09557+3521 | T-21/2020/SPOC | 120 | - | - | - | 2896 | 0.5 | 6.83 ± 0.59 | - |
| 49 | PM J12485+4933⋆ | T-15/2019/SPOC | 120 | 0.588 | 4.063[2] | 9 | 2948 | 2.1 | 11.95 ± 1.02 | 9.57 ± 1.04 |
| 50 | PM J12490+6606 | T-22/2020/SPOC | 120 | 3.197 | 5.55[4] | 14 | 2998 | 1 | 2.32 ± 0.35 | 1.39 ± 0.27 |
| 51 | PM J13417+5815⋆ | T-16/2019/SPOC | 120 | 1.709 | - | - | 2896 | 0.9 | 5.66 ± 0.84 | 3.72 ± 1.07 |
| 52 | PM J16591+2058⋆ | T-25/2020/SPOC | 120 | 4.075 | - | - | 2948 | 4.2 | 6.92 ± 0.59 | 4.86 ± 0.82 |

a : References- 1. Messina et al. (2017), 2. Houdebine et al. (2016), 3. Vidotto et al. (2014), 4. Magaudda et al. (2020), 5. Newton et al. (2017), 6. Kiraga (2012), 7. Schöfer et al. (2019), 8. Stelzer et al. (2022), 9. Rodríguez Martínez et al. (2020), 10. Raetz et al. (2020), 11. Newton et al. (2016), 12. Günther et al. (2020), 13. Newton et al. (2018), 14. Houdebine et al. (2017).

b: Sources having different rotation periods from this study, computed with the following method: 1. This was estimated by the empirical relation between Chromospheric activity and rotation period, 2. This was estimated by using All Sky Automated Survey (ASAS) photometry data (having low cadence; mostly one data point per day), 3. This was estimated by Hungarian-made Automated Telescope Network (HATNet) survey photometry data (they studied 1568 stars), 4. This was estimated with the help of v-sin$i$ and the radius of the star, where the star's radius was calculated using empirical relation, 5. Messina et al. (2016) estimated this rotation period using their own photometry observation of this previously known visual binary stars, 6. This was estimated by using photometry data from MEarth (having cadence of 30 minutes; they studied 387 stars).

Table 3: Continue...

| Source ID | Source name | Mission/Year/Author | Exposure time (s) | Rotation period (days) | Rotation Period from literature[b] (days) | Ref.[a] | $T_{spot}$ (K) | Filling factor % | Mean FLI Hα | Mean FLI Hβ |
|---|---|---|---|---|---|---|---|---|---|---|
| 53 | PM J00325+0729 | T-42/2021/SPOC | 120 | 1.820 | 3.355,0.925[5] | 1 | 2845 | 11.3 | 9.89 ± 0.63 | 6.41 ± 0.80 |
| 54 | PM J01593+5831 | - | - | - | 4.144 | 9 | 2845 | - | 9.41 ± 0.72 | 7.90 ± 0.90 |
| 55 | PM J02088+4926* | T-18/2019/SPOC | 120 | 0.749 | 0.748 | 7 | 2896 | 4.1 | 15.00 ± 1.37 | 11.00 ± 1.28 |
| 56 | PM J05062+0439 | T-05/2018/SPOC | 120 | 0.889 | 0.889 | 6 | 2845 | 4 | 10.80 ± 0.87 | 9.28 ± 1.42 |
| 57 | PM J06000+0242* | T-33/2020/SPOC | 20 | 1.807 | 1.809 | 5 | 2845 | 1.1 | 4.89 ± 0.49 | 3.72 ± 0.67 |
| 58 | PM J07033+3441* | T-20/2019/SPOC | 120 | - | 0.889 | 11 | 2845 | 3.4 | 8.59 ± 0.66 | 6.95 ± 0.87 |
| 59 | PM J07100+3831 | T-20/2019/SPOC | 120 | 5.483 | 5.593 | 5 | 2792 | 1.7 | 2.44 ± 0.22 | 1.39 ± 0.33 |
| 60 | PM J09161+0153* | T-08/2019/SPOC | 120 | 1.432 | 4.308[2] | 9 | 2896 | 8.2 | 8.61 ± 0.77 | 6.44 ± 1.39 |
| 61 | PM J10357+0215 | K-14/2017/K2 | 1800 | 0.707 | - | - | 2948 | 4 | 6.56 ± 1.40 | 1.98 ± 0.89 |
| 62 | PM J10360+0507 | - | - | - | 6.843 | 9 | 2896 | - | 10.42 ± 0.62 | 8.04 ± 1.56 |
| 63 | PM J11033+1337 | T-22/2020/SPOC | 120 | - | 34.42 | 5 | 2896 | 0.5 | 6.03 ± 0.64 | - |
| 64 | PM J11118+3332S* | T-22/2020/SPOC | 120 | 7.763 | 7.770 | 5 | 2896 | 9.3 | 10.39 ± 1.28 | 6.93 ± 3.01 |
| 65 | PM J12156+5239 | T-22/2020/SPOC | 120 | 0.726 | 4.891[2] | 9 | 2948 | 3.4 | 12.16 ± 0.94 | 10.23 ± 2.09 |
| 66 | PM J13536+7737* | T-41/2021/SPOC | 120 | 1.231 | 1.231 | 5 | 2792 | 2 | 6.78 ± 1.44 | 3.09 ± 2.02 |
| 67 | PM J14165-0725* | - | - | - | - | - | 2948 | - | 7.61 ± 0.68 | 3.50 ± 1.13 |
| 68 | PM J15126+4543* | T-24/2020/SPOC | 120 | 1.687 | 1.686 | 5 | 2845 | 3.9 | 6.64 ± 0.80 | 4.22 ± 1.41 |
| 69 | PM J05243-1601* | T-32/2020/SPOC | 120 | 0.396 | 0.401 | 1 | 2739 | 15.9 | 11.90 ± 1.15 | 10.24 ± 1.73 |
| 70 | PM J13317+2916 | T-23/2020/SPOC | 120 | 0.268 | 0.268 | 11 | 2845 | 3.5 | 14.97 ± 0.87 | 13.42 ± 2.09 |
| 71 | PM J17199+2630W | T-25/2020/SPOC | 120 | - | 19.808 | 5 | 2845 | 5.7 | 4.20 ± 0.27 | 2.27 ± 0.57 |
| 72 | PM J01033+6221 | T-24/2020/SPOC | 120 | 1.027 | 1.024 | 5 | 2739 | 20.1 | 16.70 ± 1.19 | 18.53 ± 3.05 |
| 73 | PM J02002+1303 | - | - | - | 0.199 | 11 | 2792 | - | 2.62 ± 0.27 | 1.10 ± 0.64 |
| 74 | PM J06579+6219 | T-20/2019/SPOC | 120 | 2.587 | 54.5[6] | 5 | 2739 | 1.6 | 3.12 ± 0.42 | 1.57 ± 0.98 |
| 75 | PM J07364+0704* | T-34/2021/SPOC | 20 | 0.571 | 0.996[6] | 11 | 2739 | 0.6 | 6.20 ± 0.60 | 5.85 ± 1.13 |
| 76 | PM J09449-1220* | T-35/2021/SPOC | 120 | 0.442 | 0.442 | 6 | 2845 | 14.9 | 14.35 ± 1.51 | 16.30 ± 7.87 |
| 77 | PM J12142+0037* | K-102/2016/K2SFF | 1800 | 1.584 | 1.583 | 5 | 2792 | 5.1 | 7.77 ± 0.67 | 6.41 ± 2.18 |
| 78 | PM J13005+0541* | T-23/2020/SPOC | 120 | 0.600 | 0.6 | 5 | 2792 | 2.9 | 9.82 ± 0.88 | 7.06 ± 1.57 |
| 79 | PM J20298+0941* | - | - | - | 0.257 | 5 | 2739 | - | 7.88 ± 1.32 | 5.05 ± 2.44 |
| 80 | PM J12332+0901 | T-23/2020/SPOC | 120 | 0.207 | - | - | 2845 | 1.5 | 6.39 ± 0.37 | 7.62 ± 1.28 |
| 81 | PM J17338+1655* | T-26/2020/SPOC | 120 | 0.266 | 0.266 | 5 | 2739 | 18.5 | 15.48 ± 1.28 | 9.33 ± 1.15 |
| 82 | PM J10564+0700* | K-14/2017/K2SFF | 1800 | - | - | - | 2739 | 6.2 | 6.53 ± 0.71 | 10.03 ± 2.96 |
| 83 | PM J11055+4331* | T-21/2020/QLP | 1800 | - | 0.780 | 3 | 2739 | - | 9.58 ± 1.62 | 5.63 ± 1.37 |

Table 4: The derived rotation periods and star-spot filling factors for 31 sources of Lee et al. (2010). The $T_{\rm eff}$ values for these sources are estimated from $T_{\rm eff}$ versus spectral type relation given in Rajpurohit et al. (2013).

| Source name | Mission/Year/ Author | Exposure time (s) | Rotation period (days) | Rotation Period from literature (days) | Ref. | $T_{eff}$ (K) | $T_{spot}$ (K) | Filling factor % |
|---|---|---|---|---|---|---|---|---|
| G99-049 | T-33/2020/SPOC | 120 | 1.805 | 1.809 | 5 | 3100 | 2792 | 1.2 |
| LHS1723 | T-32/2020/SPOC | 20 | - | 88.5 | 5 | 3100 | 2792 | 0.5 |
| L449-1 | T-32/2020/SPOC | 120 | 1.296 | - | - | 3100 | 2792 | 2 |
| GL285 | T-34/2021/SPOC | 120 | 2.770 | 2.77 | 3 | 3000 | 2739 | 4.52 |
| 2MASSWJ1013426-275958 | T-09/2019/SPOC | 120 | 1.163 | - | - | 2900 | 2685 | 3.8 |
| DENIS-PJ213422.2-431610 | T-28/2020/SPOC | 120 | - | - | - | 2800 | 2630 | 0.5 |
| 2MASSJ02591181+0046468 | T-04/2018/SPOC | 120 | - | - | - | 2800 | 2630 | 0.8 |
| 2MASSJ02534448-7959133 | T-39/2021/SPOC | 120 | - | - | - | 2800 | 2630 | 1.8 |
| 2MASSJ00244419-2708242 | T-29/2020/SPOC | 120 | 0.945 | 0.9432 | 12 | 2800 | 2630 | 11.3 |
| 2MASSJ00045753-1709369 | T-29/2020/SPOC | 120 | 0.192 | 0.192157 | 12 | 2800 | 2630 | 1.9 |
| 2MASSJ20021341-5425558 | T-27/2020/SPOC | 120 | 0.692 | - | - | 2800 | 2630 | 4.4 |
| LP844-25 | T-35/2021/SPOC | 120 | - | - | - | 2800 | 2630 | 2.9 |
| 2MASSJ23373831-1250277 | T-42/2021/SPOC | 120 | - | 4.9705 | 12 | 2800 | 2630 | 7.3 |
| 2MASSWJ1012065-304926 | T-36/2021/SPOC | 120 | 0.724 | - | - | 2800 | 2630 | 3.5 |
| LP731-47 | T-36/2021/SPOC | 120 | - | 0.588 | 13 | 2800 | 2630 | 3.6 |
| 2MASSJ23155449-0627462 | T-42/2021/SPOC | 120 | 0.127 | - | - | 2800 | 2630 | 4.1 |
| GJ3622 | T-09/2019/SPOC | 120 | - | - | - | 2700 | 2575 | 0.9 |
| 2MASSJ05023867-3227500 | T-32/2020/SPOC | 120 | 0.759 | - | - | 2700 | 2575 | 5 |
| 2MASSJ02141251-0357434 | T-31/2020/SPOC | 120 | 2.296 | 2.33 | 13 | 2700 | 2575 | 6 |
| 2MASSJ10031918-0105079 | T-08/2019/TESS-SPOC | 1800 | 0.213 | - | - | 2700 | 2575 | 21.8 |
| 2MASSJ13092185-2330350 | T-10/2019/SPOC | 120 | - | - | - | 2700 | 2575 | 2.8 |
| 2MASSWJ1420544-361322 | T-11/2019/SPOC | 120 | - | - | - | 2700 | 2575 | 8.6 |
| 2MASSJ09522188-1924319 | T-35/2021/SPOC | 120 | 0.909 | - | - | 2600 | 2519 | 41.6 |
| 2MASSJ04291842-3123568 | T-32/2020/SPOC | 120 | 0.907 | - | - | 2600 | 2519 | 3.6 |
| 2MASSJ23062928-0502285 | K-19/2018/K2 | 1800 | - | 3.29 | 7 | 2600 | 2519 | - |
| 2MASSJ03313025-3042383 | T-31/2020/SPOC | 120 | 1.043 | - | - | 2600 | 2519 | 3.9 |
| 2MASSJ04351612-1606574 | T-32/2020/SPOC | 120 | 0.622 | - | - | 2600 | 2519 | 3 |
| 2MASSJ02484100-1651216 | T-31/2020/SPOC | 120 | - | - | - | 2600 | 2519 | 3.9 |
| 2MASSJ22264440-7503425 | T-27/2020/SPOC | 120 | 0.678 | - | - | 2500 | 2462 | 10.4 |
| 2MASSJ03061159-3647528 | T-31/2020/SPOC | 120 | 0.294 | - | - | 2500 | 2462 | 8.4 |
| 2MASSJ23312174-2749500 | T-29/2020/SPOC | 120 | 0.431 | 0.4304 | 12 | 2500 | 2462 | 8.2 |

Table 5: Details presented in this table are used to determine the age (last column) of our sources. The coordinates RA, DEC and J,H,K magnitudes are taken from SIMBAD and all other parameters taken from Gaia Data Release 3 (Gaia Collaboration et al., 2022).

| Source ID | RA (hh:mm:ss) | DEC (dd:mm:ss) | J | H | K | *g* | *bp* | *rp* | Proper motion in RA (mas year$^{-1}$) | Proper motion in DEC (mas year$^{-1}$) | Radial velocity (km s$^{-1}$) | Parallaxes (mas) | Age (Gyr) |
|---|---|---|---|---|---|---|---|---|---|---|---|---|---|
| 1 | 03 33 14.04 | +46 15 18.97 | 8.382 | 7.770 | 7.592 | 10.497 | 11.305 | 9.590 | 68.9023 ± 0.0146 | -172.5847 ± 0.0146 | -14.2682± 8.3249 | 27.4809 ± 0.0158 | 4.681 ± 1.247 |
| 2 | 03 41 37.27 | +55 13 06.83 | 8.347 | 7.649 | 7.499 | 10.557 | 11.469 | 9.607 | 96.7821 ± 0.0149 | -116.6387 ± 0.0155 | -4.6260 ± 0.3481 | 27.9199 ± 0.0145 | 4.904 ± 2.104 |
| 3 | 07 15 08.78 | +15 55 44.95 | 8.741 | 8.144 | 7.973 | 10.972 | 11.686 | 10.007 | 209.7643 ± 0.0247 | -169.0688 ± 0.0206 | 21.2126 ± 29.2719 | 18.9026 ± 0.0207 | 2.493 ± 5.213 |
| 4 | 23 08 19.55 | -15 24 35.76 | 7.979 | 7.301 | 7.114 | 10.186 | 11.151 | 9.209 | 107.0280 ± 0.0284 | -18.8887 ± 0.0231 | -1.1762 ± 4.3937 | 40.0995 ± 0.0235 | 1.872 ± 1.411 |
| 5 | 03 32 13.32 | +49 14 21.12 | 8.989 | 8.320 | 8.114 | 11.227 | 12.195 | 10.246 | 23.3750 ± 0.0199 | -71.1782 ± 0.0210 | 11.6220 ± 0.5294 | 25.7423 ± 0.0238 | 0.672 ± 0.245 |
| 6 | 04 59 34.83 | +01 47 00.66 | 7.117 | 6.450 | 6.261 | 9.322 | 10.259 | 8.357 | 39.1302 ± 0.0149 | -94.9004 ± 0.0124 | 18.5395 ± 0.2543 | 40.9899 ± 0.0128 | - |
| 7 | 10 14 19.16 | +21 04 29.81 | 7.074 | 6.448 | 6.261 | 9.369 | 10.300 | 8.405 | - | - | -0.2496 ± 7.3263 | - | 5.846 ± 3.787 |
| 8 | 19 02 40.12 | +32 31 33.00 | 8.606 | 7.946 | 7.763 | 10.785 | 11.681 | 9.847 | 80.5793 ± 0.0111 | 44.9637 ± 0.0121 | -13.1832± 2.1615 | 27.3414 ± 0.0106 | 12.505 ± 6.259 |
| 9 | 23 06 04.84 | +63 55 34.35 | 7.815 | 7.167 | 6.977 | 10.144 | 11.119 | 9.170 | 173.6033 ± 0.0131 | -59.0774 ± 0.0134 | -25.1527± 0.3088 | 41.6161 ± 0.0125 | 10.225 ± 1.666 |
| 10 | 06 31 01.15 | +50 02 48.23 | 7.873 | 7.246 | 7.063 | 10.264 | 11.343 | 9.234 | -109.5240 ± 0.0172 | -169.0901 ± 0.0147 | 7.2223 ± 0.7863 | 48.5760 ± 0.0170 | 2.608 ± 3.956 |
| 11 | 08 31 47.92 | +05 45 18.41 | 8.915 | 8.230 | 8.080 | 11.209 | 12.191 | 10.219 | -28.4405 ± 0.1294 | -88.8624 ± 0.1162 | 13.6689 ± 1.7486 | 20.6306 ± 0.1210 | 5.522 ± 3.431 |
| 12 | 09 19 22.86 | +62 03 16.89 | 8.168 | 7.487 | 7.317 | 10.514 | 11.530 | 9.494 | -288.0994 ± 0.0175 | -386.0978 ± 0.0195 | - | 26.3567 ± 0.0205 | - |
| 13 | 12 57 40.25 | +35 13 29.62 | 7.401 | 6.734 | 6.552 | 9.772 | 10.808 | 8.758 | -277.6478 ± 0.2049 | -107.8261 ± 0.1493 | -8.8308 ± 0.5765 | 56.1107 ± 0.2844 | 3.43 ± 3.284 |
| 14 | 15 23 53.86 | +56 09 32.09 | 8.794 | 8.095 | 7.951 | 10.980 | 11.920 | 10.010 | 79.4254 ± 0.0133 | -40.0067 ± 0.0136 | -2.1499 ± 14.6487 | 19.7023 ± 0.0113 | - |
| 15 | 15 58 10.29 | +49 27 08.28 | 8.732 | 8.018 | 7.873 | 11.220 | 12.254 | 10.192 | 68.9517 ± 0.0243 | -176.8214 ± 0.0260 | -8.9740 ± 2.9137 | 26.3621 ± 0.0208 | 6.702 ± 1.465 |
| 16 | 04 37 37.45 | -02 29 28.95 | 7.299 | 6.639 | 6.413 | 9.801 | 10.816 | 8.693 | 54.7825 ± 0.4970 | -47.3122 ± 0.3928 | 21.4396 ± 0.3165 | 36.0085 ± 0.4758 | - |
| 17 | 00 42 48.24 | +35 32 55.65 | 7.164 | 6.506 | 6.321 | 9.562 | 10.643 | 8.525 | 262.0414 ± 0.0161 | 77.8809 ± 0.0146 | 2.6326 ± 7.5571 | 46.1253 ± 0.0189 | - |
| 18 | 05 40 16.09 | +12 39 00.62 | 8.072 | 7.409 | 7.199 | 10.454 | 11.527 | 9.419 | -16.5736 ± 0.0216 | -260.8613 ± 0.0152 | - | 29.0684 ± 0.0212 | - |
| 19 | 06 26 14.53 | +23 49 38.56 | 8.640 | 7.960 | 7.748 | 10.996 | 12.088 | 9.956 | -10.7880 ± 0.0203 | -136.2338 ± 0.0170 | 16.1854 ± 0.3159 | 36.3393 ± 0.0232 | 1.275 ± 0.157 |
| 20 | 07 29 31.09 | +35 56 00.38 | 8.644 | 7.998 | 7.796 | 11.054 | 12.122 | 10.022 | -42.4054 ± 0.1974 | -114.9698 ± 0.1550 | 12.3812 ± 1.8239 | 23.4217 ± 0.2012 | 0.025 ± 0 |
| 21 | 13 00 46.55 | +12 22 32.67 | 6.437 | 5.786 | 5.578 | 8.899 | 9.993 | 7.846 | -628.7153 ± 0.1842 | -33.4718 ± 0.1326 | -12.3258± 0.3233 | 86.9010 ± 0.1170 | 7.265 ± 2.733 |
| 22 | 15 41 37.24 | +18 28 08.20 | 8.955 | 8.295 | 8.062 | 11.379 | 12.481 | 10.323 | -65.0547 ± 0.1421 | 64.8903 ± 0.0990 | -20.8933± 7.7121 | 19.3668 ± 0.1390 | - |
| 23 | 16 22 01.17 | +22 50 21.74 | 8.904 | 8.271 | 8.094 | 11.347 | 12.425 | 10.308 | -51.7634 ± 0.0903 | 68.1566 ± 0.1190 | -33.0982± 2.0618 | 19.1658 ± 0.1095 | - |
| 24 | 22 38 45.57 | -20 37 16.08 | 5.669 | 5.108 | 4.800 | 8.170 | 9.348 | 7.083 | 449.2068 ± 0.0504 | -79.0459 ± 0.0462 | - | 112.3859± 0.0555 | 3.205 ± 0.256 |
| 25 | 04 28 28.77 | +17 41 45.39 | 8.592 | 7.956 | 7.711 | 11.360 | 12.490 | 10.255 | 109.4870 ± 0.4488 | -44.2273 ± 0.2935 | 32.1318 ± 1.5401 | 20.9184 ± 0.4034 | - |
| 26 | 06 21 13.03 | +44 14 30.73 | 8.724 | 8.081 | 7.885 | 11.306 | 12.475 | 10.207 | 151.7723 ± 0.0288 | -252.2423 ± 0.0232 | - | 26.9255 ± 0.0304 | 0.025 ± 0 |
| 27 | 11 20 06.10 | -10 29 46.72 | 7.814 | 7.210 | 6.967 | 10.303 | 11.462 | 9.224 | -197.8889 ± 0.0478 | 19.8403 ± 0.0437 | 11.1384 ± 0.3450 | 52.8248 ± 0.0378 | 7.782 ± 3.989 |
| 28 | 13 51 52.91 | +12 47 07.12 | 8.788 | 8.184 | 7.970 | 11.260 | 12.406 | 10.192 | 91.1158 ± 0.0291 | -10.1799 ± 0.0226 | -7.3186 ± 0.4620 | 37.5069 ± 0.0309 | 1.297 ± 3.294 |
| 29 | 15 21 52.93 | +20 58 39.91 | 6.610 | 5.960 | 5.756 | 9.124 | 10.273 | 8.053 | 81.5028 ± 0.0233 | 128.0782 ± 0.0219 | 5.3064 ± 3.6760 | 87.3251 ± 0.0214 | 7.325 ± 0.239 |
| 30 | 16 17 05.35 | +55 16 08.77 | 6.600 | 5.992 | 5.770 | 9.078 | 10.184 | 8.015 | 87.9699 ± 0.6007 | -430.9627 ± 0.5423 | -32.8097± 1.6573 | 49.6303 ± 0.4245 | - |
| 31 | 06 59 41.57 | +05 45 39.96 | 8.947 | 8.370 | 8.060 | 11.467 | 12.677 | 10.375 | -19.1684 ± 0.0262 | -67.6569 ± 0.0216 | 11.8528 ± 0.4858 | 34.3813 ± 0.0230 | 8.002 ± 0.343 |
| 32 | 09 17 44.71 | +46 12 24.66 | 8.126 | 7.490 | 7.245 | 10.942 | 11.812 | 9.552 | - | - | - | - | - |
| 33 | 10 04 21.46 | +50 23 13.38 | 8.081 | 7.413 | 7.199 | 10.615 | 11.857 | 9.507 | -141.0791 ± 0.0159 | -202.3356 ± 0.0156 | -1.5916 ± 0.6745 | 45.8541 ± 0.0188 | 0.832 ± 1.975 |
| 34 | 11 51 56.82 | +07 31 26.52 | 8.812 | 8.130 | 7.887 | 11.408 | 12.594 | 10.321 | -126.4511 ± 0.0304 | -81.6837 ± 0.0233 | - | 19.7052 ± 0.0280 | - |
| 35 | 15 55 47.22 | +68 40 13.85 | 8.593 | 7.962 | 7.752 | 11.129 | 12.344 | 10.032 | -44.3376 ± 0.0182 | 132.8493 ± 0.0199 | -17.4758± 0.4882 | 39.0421 ± 0.0149 | 6.325 ± 1.019 |
| 36 | 04 33 23.76 | +23 59 27.07 | 8.914 | 8.242 | 8.028 | 12.344 | 12.892 | 10.507 | 92.1744 ± 0.5887 | -55.5093 ± 0.4628 | 39.4231 ± 3.9189 | 19.4879 ± 0.5391 | - |
| 37 | 05 09 09.96 | +15 27 32.91 | 8.770 | 8.247 | 7.961 | 11.428 | 12.730 | 10.299 | 135.9864 ± 0.0539 | -634.8353 ± 0.0389 | -21.9520± 2.0624 | 33.5675 ± 0.0432 | 12.355 ± 1.295 |
| 38 | 05 33 44.80 | +01 56 43.45 | 7.764 | 7.150 | 6.855 | 10.380 | 11.681 | 9.250 | -231.5393 ± 0.0450 | -153.9888 ± 0.0367 | 48.5729 ± 7.6240 | 63.3597 ± 0.0477 | 4.223 ± 3.069 |
| 39 | 05 54 45.73 | +10 55 57.01 | 8.832 | 8.213 | 7.970 | 11.431 | 12.728 | 10.304 | -140.2558 ± 0.0342 | -69.3583 ± 0.0266 | 12.7598 ± 3.3766 | 40.5364 ± 0.0288 | 8.866 ± 2.989 |
| 40 | 07 31 57.71 | +36 13 09.79 | 6.771 | 6.179 | 5.927 | 9.601 | 10.869 | 8.410 | -249.6772 ± 0.0569 | -247.1195 ± 0.0539 | -0.7938 ± 0.5721 | 83.3788 ± 0.0487 | 1.9 ± 1.098 |
| 41 | 07 34 56.32 | +14 45 53.80 | 7.287 | 6.679 | 6.398 | 10.440 | 11.484 | 8.993 | -73.6966 ± 0.0890 | -80.2302 ± 0.0740 | - | 61.3671 ± 0.0847 | - |
| 42 | 11 52 57.14 | +35 54 45.98 | 9.962 | 9.354 | 9.128 | 12.636 | 13.957 | 11.498 | -99.8610 ± 0.0196 | 23.7983 ± 0.0237 | -8.7611 ± 2.5992 | 25.1421 ± 0.0265 | 8.734 ± 0.917 |
| 43 | 12 35 33.44 | +24 39 18.32 | 9.933 | 9.254 | 9.057 | 12.439 | 13.620 | 11.355 | -95.2269 ± 0.0477 | -3.5007 ± 0.0405 | -10.3480± 6.5201 | 13.6839 ± 0.0507 | - |
| 44 | 13 35 12.46 | +17 14 08.91 | - | - | 12.297 | 13.335 | 11.213 | -15.945 | -61.3969 ± 0.1755 | -15.9447 ± 0.1191 | -17.8390± 4.3528 | 13.5958 ± 0.1815 | - |
| 45 | 14 13 46.73 | +46 18 22.83 | 9.431 | 8.802 | 8.591 | 12.075 | 13.316 | 10.963 | -138.7868 ± 0.0157 | 10.8266 ± 0.0196 | -15.4743± 2.9022 | 25.4881 ± 0.0183 | 1.305 ± 1.621 |
| 46 | 04 23 50.37 | +14 55 17.50 | 9.293 | 8.718 | 8.454 | 12.135 | 13.560 | 10.953 | 113.9473 ± 0.2356 | -28.7256 ± 0.1983 | 38.4325 ± 1.6550 | 25.6599 ± 0.2145 | 1.662 ± 2.955 |
| 47 | 09 30 14.42 | +26 30 24.86 | 8.866 | 8.284 | 8.020 | 11.647 | 13.057 | 10.463 | -154.2215 ± 0.0360 | -136.9053 ± 0.0297 | 19.9947 ± 0.3000 | 41.3081 ± 0.0327 | 1.067 ± 0.906 |
| 48 | 09 55 43.59 | +35 21 41.76 | 8.850 | 8.297 | 8.043 | 11.615 | 13.017 | 10.443 | -35.9753 ± 0.0327 | -312.7036 ± 0.0279 | -11.0347± 0.3952 | 52.1159 ± 0.0329 | 5.369 ± 1.039 |
| 49 | 12 48 34.49 | +49 33 54.02 | 8.680 | 8.019 | 7.775 | 11.349 | 12.747 | 10.183 | 108.5818 ± 0.3276 | -16.9214 ± 0.4152 | -11.4651± 1.0125 | 37.2245 ± 0.4569 | 6.868 ± 6.151 |
| 50 | 12 49 02.75 | +66 06 36.66 | 6.880 | 6.299 | 6.070 | 9.844 | 11.153 | 8.517 | - | - | - | - | 6.581 ± 4 |
| 51 | 13 41 46.30 | +58 15 19.79 | 8.730 | 8.171 | 7.876 | 11.816 | 12.864 | 10.299 | 81.7750 ± 0.0671 | -59.3569 ± 0.0705 | -10.5501± 0.7238 | 46.2510 ± 0.0633 | - |
| 52 | 16 59 09.62 | +20 58 16.03 | 8.338 | 7.745 | 7.513 | 11.504 | 12.638 | 9.983 | -23.4469 ± 0.0551 | 117.7281 ± 0.0602 | - | 50.7728 ± 0.0727 | - |
| 53 | 00 32 34.79 | +07 29 26.95 | 8.397 | 7.790 | 7.508 | 11.653 | 12.869 | 10.111 | 104.3635 ± 0.0844 | -62.9113 ± 0.0550 | - | 28.4343 ± 0.0606 | - |
| 54 | 01 59 23.51 | +58 31 16.10 | 7.790 | 7.224 | 6.961 | 10.846 | 12.493 | 9.599 | 320.6190 ± 0.0221 | -192.6339 ± 0.0257 | -9.5920 ± 0.3575 | 76.2912 ± 0.0252 | 3.476 ± 2.797 |
| 55 | 02 08 53.62 | +49 26 56.43 | 8.423 | 7.811 | 7.584 | 11.273 | 12.744 | 10.081 | 236.4287 ± 0.0307 | -291.1776 ± 0.0397 | -11.2394± 1.4607 | 58.5108 ± 0.0284 | 6.06 ± 0.399 |
| 56 | 05 06 12.92 | +04 39 27.18 | 8.909 | 8.341 | 8.067 | 11.992 | 13.669 | 10.735 | 30.1573 ± 0.0301 | -89.8644 ± 0.0220 | 20.1320 ± 3.7348 | 36.1922 ± 0.0277 | - |
| 57 | 06 00 03.50 | +02 42 23.59 | 6.905 | 6.308 | 6.042 | 9.901 | 11.545 | 8.654 | 309.1462 ± 0.0340 | -40.3684 ± 0.0241 | 29.9568 ± 0.1742 | 192.0135± 0.0310 | - |
| 58 | 07 03 23.16 | +34 41 51.39 | 8.773 | 8.178 | 7.914 | 11.760 | 13.396 | 10.523 | -57.3475 ± 0.0306 | 140.5885 ± 0.0269 | 2.9541 ± 0.3558 | 75.3464 ± 0.0282 | 2.725 ± 3.683 |
| 59 | 07 10 01.83 | +38 31 46.08 | 6.731 | 6.152 | 5.846 | 9.935 | 11.748 | 8.642 | -439.4204 ± 0.0656 | -944.7935 ± 0.0588 | - | 165.2147± 0.0636 | - |
| 60 | 09 16 10.18 | +01 53 08.83 | 8.770 | 8.260 | 7.960 | 11.689 | 13.238 | 10.474 | 54.8226 ± 0.0314 | -101.3046 ± 0.0221 | -13.2892± 0.7584 | 63.8909 ± 0.0276 | 5.469 ± 0.887 |
| 61 | 10 35 46.92 | +02 15 58.31 | 9.827 | 9.217 | 8.969 | 12.818 | 13.751 | 11.342 | - | - | - | - | - |
| 62 | 10 36 01.21 | +05 07 12.79 | 8.463 | 7.875 | 7.598 | 11.367 | 12.913 | 10.142 | -654.1207 ± 0.0654 | 127.5107 ± 0.0570 | 20.1588 ± 0.5059 | 65.4708 ± 0.0494 | 12.528 ± 4.895 |
| 63 | 11 03 21.25 | +13 37 57.02 | 8.759 | 8.181 | 7.914 | 11.663 | 13.248 | 10.440 | -193.0805 ± 0.0880 | 76.5425 ± 0.0839 | -4.6812 ± 37.9577 | 65.8437 ± 0.0701 | 12.344 ± 1.128 |
| 64 | 11 11 51.74 | +33 32 11.22 | 8.297 | 7.758 | 7.497 | 11.136 | 12.629 | 9.938 | -175.9738 ± 0.0264 | 116.5472 ± 0.0263 | 1.2029 ± 0.3456 | 74.8839 ± 0.0311 | - |
| 65 | 12 15 39.36 | +52 39 08.75 | 8.588 | 7.990 | 7.757 | 11.373 | 12.798 | 10.190 | 105.2421 ± 0.1172 | -1.1247 ± 0.1365 | -8.8987 ± 1.2949 | 39.8459 ± 0.1556 | 6.771 ± 1.094 |
| 66 | 13 53 38.79 | +77 37 08.15 | 8.635 | 8.056 | 7.795 | 11.540 | 13.123 | 10.320 | 224.2460 ± 0.0256 | -15.1233 ± 0.0250 | -7.2600 ± 0.4172 | 75.4803 ± 0.0225 | 5.482 ± 2.438 |
| 67 | 14 16 33.29 | -07 25 38.32 | 9.812 | 9.204 | 8.940 | 12.591 | 13.974 | 11.434 | 42.7499 ± 0.0279 | -36.2417 ± 0.0215 | -3.6663 ± 16.5325 | 17.2821 ± 0.0235 | - |
| 68 | 15 12 38.18 | +45 43 46.87 | 8.977 | 8.392 | 8.108 | 12.280 | 13.603 | 10.716 | -385.9276 ± 0.4879 | 338.9428 ± 0.5977 | -9.5640 ± 1.1823 | 52.5864 ± 0.4881 | - |
| 69 | 05 24 19.13 | -16 01 15.27 | 8.668 | 8.130 | 7.807 | 12.497 | 13.788 | 10.622 | 31.9866 ± 0.7272 | -24.0030 ± 0.7616 | 27.4746 ± 3.2101 | 32.0614 ± 0.7951 | - |
| 70 | 13 31 46.62 | +29 16 36.68 | 7.561 | 7.002 | 6.720 | 10.628 | 12.256 | 9.362 | - | - | -8.9358 ± 1.6198 | - | 6.131 ± 4.015 |
| 71 | 17 19 54.20 | +26 30 03.06 | 7.273 | 6.710 | 6.422 | 10.148 | 11.630 | 8.949 | -214.8369 ± 0.0218 | 350.8502 ± 0.0274 | -35.5909± 1.7444 | 92.9857 ± 0.0252 | - |
| 72 | 01 03 19.83 | +62 21 55.83 | 8.611 | 8.014 | 7.718 | 11.927 | 13.900 | 10.594 | 730.3980 ± 0.0387 | 85.9667 ± 0.0453 | - | 101.3724± 0.0480 | - |
| 73 | 02 00 12.95 | +13 03 07.00 | 7.514 | 6.970 | 6.648 | 10.681 | 12.572 | 9.384 | 1096.4585 ± 0.0667 | -1771.5261 ± 0.0566 | -28.2924± 0.2548 | 223.7321± 0.0699 | - |
| 74 | 06 57 57.11 | +62 19 19.36 | 8.585 | 7.988 | 7.690 | 12.149 | 13.946 | 10.676 | 298.6085 ± 0.0367 | -536.5402 ± 0.0344 | - | 87.0311 ± 0.0496 | 4.453 ± 0.864 |
| 75 | 07 36 25.11 | +07 04 43.13 | 8.180 | 7.611 | 7.282 | 12.014 | 13.498 | 10.163 | - | - | - | - | - |
| 76 | 09 44 54.19 | -12 20 54.37 | 8.496 | 7.919 | 7.601 | 11.872 | 13.925 | 10.534 | -331.3270 ± 0.0338 | 40.1774 ± 0.0373 | - | 76.0509 ± 0.0336 | - |
| 77 | 12 14 16.54 | +00 37 26.36 | 8.456 | 7.860 | 7.540 | 11.829 | 13.859 | 10.491 | -951.3357 ± 0.0564 | -284.0494 ± 0.0389 | - | 123.6430± 0.0449 | - |
| 78 | 13 00 33.52 | +05 41 07.99 | 8.553 | 7.966 | 7.660 | 11.773 | 13.656 | 10.468 | -940.6305 ± 0.0812 | 227.7496 ± 0.0708 | -27.4927± 0.6098 | 117.0327± 0.0613 | - |
| 79 | 20 29 48.31 | +09 41 20.59 | 8.228 | 7.666 | 7.307 | 11.485 | 13.337 | 10.169 | - | - | -37.6922± 19.4221 | - | 6.309 ± 3.949 |
| 80 | 12 33 17.36 | +09 01 15.79 | 6.995 | 6.397 | 6.042 | 11.240 | 13.037 | 9.540 | -1710.4677 ± 0.5542 | 203.0978 ± 0.4507 | - | 223.4775± 0.4665 | - |
| 81 | 17 33 53.17 | +16 55 13.06 | 8.895 | 8.299 | 7.995 | 12.400 | 14.557 | 11.021 | -135.0466 ± 0.4598 | -130.4698 ± 0.4449 | -15.2668± 2.2901 | 60.9122 ± 0.4797 | - |
| 82 | 10 56 28.92 | +07 00 53.00 | 7.085 | 6.482 | 6.084 | 11.038 | 13.770 | 9.585 | -3866.3383 ± 0.0813 | -2699.2150 ± 0.0691 | - | 415.1794± 0.0684 | - |
| 83 | 11 05 30.88 | +43 31 17.88 | 8.742 | 8.177 | 7.839 | 12.257 | 14.710 | 10.855 | -4339.8496 ± 0.0448 | 960.6961 ± 0.0414 | 67.9359 ± 0.7406 | 203.8323± 0.0500 | 8.399 ± 4.675 |

Table 6: Details presented in this table are used to determine the age (last column) of Lee et al. (2010) sources. The coordinates RA, DEC and J,H,K magnitudes are taken from SIMBAD and all other parameters taken from Gaia Data Release 3 (Gaia Collaboration et al., 2022).

| Source Name | RA (hh:mm:ss) | DEC (dd:mm:ss) | J | H | K | $g$ | $bp$ | $rp$ | Proper motion in RA (mas year$^{-1}$) | Proper motion in DEC (mas year$^{-1}$) | Radial velocity (km s$^{-1}$) | Parallaxes (mas) | Age (Gyr) |
|---|---|---|---|---|---|---|---|---|---|---|---|---|---|
| G 99-049 | 06 00 03.50 | +02 42 23.59 | 6.905 | 6.308 | 6.042 | 9.901 | 11.545 | 8.654 | 309.1462 ± 0.0340 | -40.3684 ± 0.0241 | 29.9568 ± 0.1742 | 192.0135± 0.0310 | - |
| LHS 1723 | 05 01 57.42 | -06 56 46.37 | 7.617 | 7.065 | 6.736 | 10.649 | 12.413 | 9.380 | -551.7464 ± 0.0265 | -533.6482 ± 0.0207 | 42.2863 ± 0.1750 | 186.0466± 0.0277 | - |
| L 449-1 | 05 17 22.90 | -35 21 54.65 | 7.400 | 6.854 | 6.558 | 10.349 | 11.932 | 9.121 | -219.3826 ± 0.3094 | -166.4681 ± 0.3317 | -1.9771 ± 1.0568 | 85.4519 ± 0.2898 | 4.462 ± 2.904 |
| GJ 1224 | 18 07 32.83 | -15 57 47.06 | 8.639 | 8.085 | 7.827 | 11.863 | 13.780 | 10.560 | -618.4062 ± 0.0333 | -347.0067 ± 0.0269 | -33.2189± 0.4677 | 125.4509± 0.0306 | - |
| GL 285 | 07 44 40.17 | +03 33 08.87 | 6.581 | 6.005 | 5.698 | 9.692 | 11.417 | 8.420 | -347.7816 ± 0.0400 | -445.7018 ± 0.0249 | 25.7171 ± 0.1962 | 166.9769± 0.0343 | - |
| 2MASSW J1013426-275958 | 10 13 42.60 | -27 59 58.63 | 12.261 | 11.626 | 11.252 | 15.837 | 18.051 | 14.444 | -70.9721 ± 0.1076 | -38.9926 ± 0.0877 | - | 24.3810 ± 0.1047 | 6.592 ± 3.504 |
| GJ 1156 | 12 18 59.39 | +11 07 33.77 | 8.525 | 7.880 | 7.570 | 11.926 | 14.100 | 10.567 | -1269.7707 ± 0.0555 | 203.4441 ± 0.0333 | - | 154.6999± 0.0445 | - |
| GJ 1154A | 12 14 16.54 | +00 37 26.36 | 8.456 | 7.860 | 7.540 | 11.829 | 13.859 | 10.491 | -951.3357 ± 0.0564 | -284.0494 ± 0.0389 | - | 123.6430± 0.0449 | - |
| DENIS-P J213422.2-431610 | 21 34 22.29 | -43 16 10.64 | 10.690 | 10.035 | 9.685 | 14.275 | 16.580 | 12.896 | 147.0431 ± 0.0296 | -793.7512 ± 0.0282 | - | 59.0205 ± 0.0333 | - |
| 2MASS J02591181+0046468 | 02 59 11.81 | +00 46 46.85 | 11.725 | 11.129 | 10.863 | 14.901 | 16.803 | 13.604 | 176.5674 ± 0.0381 | -42.4316 ± 0.0331 | 34.4131 ± 5.1623 | 22.4993 ± 0.0363 | - |
| 2MASS J02534448-7959133 | 02 53 44.47 | -79 59 13.26 | 11.336 | 10.740 | 10.379 | 15.051 | 17.619 | 13.632 | 77.2420 ± 0.0525 | 84.2326 ± 0.0513 | - | 57.2108 ± 0.0378 | 6.933 ± 5.093 |
| 2MASS J00244419-2708242 | 00 24 44.17 | -27 08 25.26 | 9.254 | 8.547 | 8.241 | 13.143 | 15.553 | 11.587 | -92.7389 ± 0.1108 | 695.9562 ± 0.1171 | -28.9832± 0.7666 | 129.3167± 0.1256 | 0.831 ± 4.808 |
| 2MASS J00045753-1709369 | 00 04 57.54 | -17 09 36.95 | 10.997 | 10.455 | 10.084 | 14.582 | 16.969 | 13.196 | 144.7759 ± 0.0426 | -8.9428 ± 0.0341 | - | 58.6246 ± 0.0492 | 5.048 ± 2.755 |
| 2MASS J20021341-5425558 | 20 02 13.44 | -54 25 55.90 | 11.621 | 11.035 | 10.644 | 15.487 | 18.355 | 14.037 | 61.5745 ± 0.0455 | -365.2540 ± 0.0410 | - | 55.5167 ± 0.0526 | - |
| LP 844-25 | 08 53 56.35 | -24 46 56.44 | 12.386 | 11.879 | 11.571 | 15.796 | 18.228 | 14.408 | 611.5040 ± 0.0519 | 157.3040 ± 0.0519 | - | 38.8220 ± 0.0548 | 0.609 ± 0.168 |
| 2MASS J16142520-0251009 | 16 14 25.19 | -02 51 00.75 | 11.303 | 10.683 | 10.280 | 15.223 | 18.242 | 13.752 | -7.8084 ± 0.0827 | 367.4055 ± 0.0610 | - | 68.9493 ± 0.0835 | - |
| 2MASS J21322975-0511585 | 21 32 29.76 | -05 11 59.02 | 11.423 | 10.730 | 10.379 | 15.095 | 17.596 | 13.692 | 115.9966 ± 0.0524 | -341.4850 ± 0.0354 | - | 49.7147 ± 0.0476 | 0.22 ± 6.675 |
| 2MASS J23373831-1250277 | 23 37 38.34 | -12 50 28.36 | 11.462 | 10.830 | 10.452 | 15.320 | 17.780 | 13.803 | 192.5646 ± 0.4121 | -305.8209 ± 0.3055 | - | 37.4154 ± 0.3504 | 0.129 ± 0.037 |
| 2MASSW J1012065-304926 | 10 12 06.48 | -30 49 26.32 | 12.223 | 11.601 | 11.179 | 16.272 | 19.355 | 14.795 | -142.4917 ± 0.0646 | 36.0642 ± 0.0822 | - | 44.2132 ± 0.0656 | - |
| LP 731-47 | 11 06 56.91 | -12 44 02.73 | 11.786 | 11.188 | 10.792 | 15.942 | 18.711 | 14.352 | -358.6362 ± 0.6262 | 22.2501 ± 0.4898 | - | 41.9403 ± 0.6076 | 0.193 ± 0.047 |
| 2MASS J23155449-0627462 | 23 15 54.50 | -06 27 46.42 | 11.111 | 10.567 | 10.228 | 14.795 | 17.338 | 13.383 | 315.1335 ± 0.0540 | -44.9079 ± 0.0385 | - | 59.6358 ± 0.0409 | 1.927 ± 0.022 |
| 2MASS J20424514-0500193 | 20 42 45.17 | -05 00 19.17 | 11.449 | 10.871 | 10.539 | 15.175 | 17.867 | 13.746 | 241.0537 ± 0.0507 | 116.9923 ± 0.0369 | -17.6063± 2.9483 | 59.9682 ± 0.0481 | 1.329 ± 0.361 |
| GJ 3622 | 10 48 12.61 | -11 20 09.61 | 8.857 | 8.263 | 7.930 | 12.837 | 15.941 | 11.360 | 579.0187 ± 0.0658 | -1530.0765 ± 0.0576 | 1.4739 ± 0.6710 | 219.3302± 0.0602 | - |
| 2MASS J05023867-3227500 | 05 02 38.68 | -32 27 50.10 | 12.443 | 11.814 | 11.439 | 16.222 | 18.821 | 14.786 | 55.8091 ± 0.0473 | -164.1750 ± 0.0611 | - | 34.1292 ± 0.0504 | 5.634 ± 2.441 |
| 2MASS J02141251-0357434 | 02 14 12.56 | -03 57 43.58 | 10.481 | 9.858 | 9.485 | 14.148 | 16.666 | 12.741 | 509.6377 ± 0.0507 | -155.8128 ± 0.0428 | - | 80.0548 ± 0.0626 | - |
| 2MASS J10031918-0105079 | 10 03 19.15 | -01 05 08.00 | 12.327 | 11.667 | 11.236 | 16.527 | 19.746 | 15.012 | -498.7060 ± 0.0920 | 46.9003 ± 0.1023 | - | 50.1372 ± 0.0950 | 8.147 ± 2.340 |
| 2MASS J13092185-2330350 | 13 09 21.85 | -23 30 35.74 | 11.785 | 11.082 | 10.669 | 16.120 | 19.467 | 14.592 | 15.7296 ± 0.1006 | -383.7718 ± 0.0727 | - | 66.6038 ± 0.0976 | - |
| 2MASSW J1032136-420856 | 10 32 13.68 | -42 08 56.94 | 12.888 | 12.211 | 11.829 | 17.115 | 20.206 | 15.598 | 91.5176 ± 0.0702 | -159.2972 ± 0.0871 | - | 39.3327 ± 0.0922 | 2.375 ± 0.000 |
| 2MASSW J1420544-361322 | 14 20 54.47 | -36 13 22.26 | 11.477 | 10.843 | 10.420 | 16.146 | 18.998 | 14.144 | - | - | - | - | - |
| 2MASS J09522188-1924319 | 09 52 21.88 | -19 24 32.20 | 11.865 | 11.256 | 10.869 | 15.735 | 18.468 | 14.292 | -73.0006 ± 0.1044 | -99.4799 ± 0.1032 | - | 35.3239 ± 0.1038 | - |
| 2MASS J04291842-3123568 | 04 29 18.46 | -31 23 56.74 | 10.874 | 10.211 | 9.770 | 15.028 | 17.556 | 13.403 | 65.8199 ± 0.1493 | 99.5806 ± 0.1636 | - | 58.7935 ± 0.1420 | 11.108 ± 5.887 |
| 2MASS J23062928-0502285 | 23 06 29.36 | -05 02 29.03 | 11.354 | 10.718 | 10.296 | 15.623 | 19.006 | 14.104 | 930.7875 ± 0.0868 | -479.0375 ± 0.0705 | - | 80.2123 ± 0.0716 | - |
| 2MASS J03313025-3042383 | 03 31 30.25 | -30 42 38.82 | 11.360 | 10.700 | 10.264 | 15.628 | 19.029 | 14.109 | 51.8694 ± 0.0408 | -403.0845 ± 0.0554 | - | 79.9468 ± 0.0556 | - |
| 2MASS J04351612-1606574 | 04 35 16.14 | -16 06 57.21 | 10.406 | 9.779 | 9.352 | 14.607 | 17.921 | 13.099 | 160.0832 ± 0.1716 | 315.1396 ± 0.1683 | - | 94.3054 ± 0.2099 | - |
| 2MASS J06572547-4019134 | 06 57 25.43 | -40 19 13.76 | 12.728 | 12.132 | 11.667 | 17.796 | 20.610 | 15.586 | -107.7470 ± 0.1924 | 64.3169 ± 0.2046 | - | 29.1861 ± 0.1660 | - |
| 2MASS J05173766-3349027 | 05 17 37.69 | -33 49 03.09 | 12.004 | 11.317 | 10.832 | 16.484 | 20.002 | 14.942 | 445.8376 ± 0.0798 | -331.4433 ± 0.0943 | - | 59.4702 ± 0.0779 | - |
| 2MASS J19165762+0509021 | 19 16 57.61 | +05 09 01.60 | 9.908 | 9.226 | 8.765 | 14.303 | 17.746 | 12.775 | -598.7613 ± 0.0717 | -1366.0635 ± 0.0650 | - | 168.9537± 0.0668 | - |
| 2MASS J22062280-2047058 | 22 06 22.82 | -20 47 06.59 | 12.370 | 11.684 | 11.315 | 16.918 | 20.013 | 15.095 | - | - | - | - | 8.038 ± 4.052 |
| 2MASS J02484100-1651216 | 02 48 40.99 | -16 51 22.12 | 12.551 | 11.872 | 11.422 | 16.848 | 20.102 | 15.318 | -33.1201 ± 0.1276 | -288.8480 ± 0.1536 | - | 44.6207 ± 0.1262 | 8.264 ± 3.51 |
| 2MASS J20370715-1137569 | 20 37 07.15 | -11 37 57.34 | 12.272 | 11.629 | 11.257 | 16.389 | 19.627 | 14.879 | -2.2340 ± 0.1121 | -379.1496 ± 0.0917 | - | 46.6595 ± 0.1034 | - |
| 2MASS J22264440-7503425 | 22 26 44.41 | -75 03 42.53 | 12.353 | 11.696 | 11.246 | 16.798 | 20.282 | 15.239 | 58.7394 ± 0.0838 | 11.7791 ± 0.0923 | - | 42.6368 ± 0.0779 | - |
| 2MASS J03061159-3647528 | 03 06 11.59 | -36 47 52.85 | 11.690 | 11.068 | 10.631 | 15.994 | 19.534 | 14.460 | -172.1654 ± 0.0497 | -669.2439 ± 0.0576 | - | 75.4184 ± 0.0580 | - |
| 2MASS J23312174-2749500 | 23 31 21.74 | -27 49 49.60 | 11.646 | 11.055 | 10.651 | 15.870 | 19.514 | 14.347 | 90.3750 ± 0.0752 | 745.2837 ± 0.0715 | - | 73.3785 ± 0.0770 | - |
